# Supplementary material for: The $(2+\delta)$-dimensional theory of the electromechanics of lipid membranes: II. Balance laws
Source: arXiv:2309.03863 ancillary file (2025-02-24)
Supplement: Supplementary file 1 [file thin_film_electromechanics_SI_part2.pdf]

# Supplementary Material

## The $(2 + \delta)$-dimensional theory of the electromechanics of lipid membranes: II. Balance laws

Yannick A. D. Omar[1,‡], Zachary G. Lipel[1,§], and Kranthi K. Mandadapu[1,2,*]

[1] Department of Chemical & Biomolecular Engineering, University of California, Berkeley, CA 94720, USA
[2] Chemical Sciences Division, Lawrence Berkeley National Laboratory, CA 94720, USA

## Contents

**1 Kinematic Results** **1**
1.1 The Position and Velocity Vectors in the Eulerian Parametrization . . . . . . . . . . 2
1.2 On the Eulerian Parametrization of the Mid-Surface . . . . . . . . . . . . . . . . . . 4

**2 Polynomial Expansions of the Christoffel Symbols** **5**
2.1 Contravariant Basis Vectors . . . . . . . . . . . . . . . . . . . . . . . . . . . . . . . 5
2.2 Christoffel Symbols . . . . . . . . . . . . . . . . . . . . . . . . . . . . . . . . . . . . 7

**3 Reactive Stresses** **9**
3.1 Kirchhoff-Love Kinematics as a Constraint . . . . . . . . . . . . . . . . . . . . . . . 9
3.2 On the Truncation of Reactive Stresses . . . . . . . . . . . . . . . . . . . . . . . . . 11

**4 Three-Dimensional Angular Momentum Balance** **18**

**5 Dimension Reduction of Balance Laws** **19**
5.1 Mass Balance . . . . . . . . . . . . . . . . . . . . . . . . . . . . . . . . . . . . . . . 19
5.2 Stress Vector Expansions . . . . . . . . . . . . . . . . . . . . . . . . . . . . . . . . . 24
5.3 Linear Momentum Balance . . . . . . . . . . . . . . . . . . . . . . . . . . . . . . . . 26
5.4 Angular Momentum Balance . . . . . . . . . . . . . . . . . . . . . . . . . . . . . . . 32

**Supporting References** **33**

# 1 Kinematic Results

This section establishes two kinematic results required in the main text: In Sec. 1.1, we derive the form of the position and velocity vectors in the Eulerian description, and in Sec. 1.2, we motivate the relation between the Eulerian mid-surface parametrization $\theta^\alpha$ and the zeroth-order in-plane velocity $v_0^\alpha$.

‡yannick.omar@berkeley.edu
§zlipel@berkeley.edu
*kranthi@berkeley.edu

## 1.1 The Position and Velocity Vectors in the Eulerian Parametrization

In Sec. 2.1 of the main text, we showed that the choice of K-L kinematics implies that the position and velocity vectors of the body $\mathcal{M}$ vary at most linearly along the thickness coordinate of the Lagrangian parametrization. In the following, we discuss the functional forms of the position and velocity vectors in the Eulerian parametrization that are consistent with K-L kinematics.

First, recall from the main text that the position and velocity vectors in the Lagrangian parametrization can be written in terms of the mid-surface position vector $\hat{\boldsymbol{x}}_0(\xi^\alpha, t)$, velocity vector $\hat{\boldsymbol{v}}_0(\xi^\alpha, t)$, and normal vector $\hat{\boldsymbol{n}}(\xi^\alpha, t)$ as

$$\hat{\boldsymbol{x}}\big(\xi^i, t\big) = \hat{\boldsymbol{x}}_0(\xi^\alpha, t) + \hat{\boldsymbol{n}}(\xi^\alpha, t)\, \xi^3 \ , \tag{1}$$

$$\hat{\boldsymbol{v}}\big(\xi^i, t\big) = \frac{\partial}{\partial t}\hat{\boldsymbol{x}}\big(\xi^i, t\big)\bigg|_{\xi^k} \tag{2}$$

$$= \hat{\boldsymbol{v}}_0(\xi^\alpha, t) + \hat{\boldsymbol{v}}_1(\xi^\alpha, t)\, \xi^3 \ , \tag{3}$$

where the mid-surface and first-order velocities $\boldsymbol{v}_0$ and $\boldsymbol{v}_1$ are given by

$$\hat{\boldsymbol{v}}_0(\xi^\alpha, t) = \frac{\partial}{\partial t}\hat{\boldsymbol{x}}_0(\xi^\alpha, t)\bigg|_{\xi^\gamma} \ , \tag{4}$$

$$\hat{\boldsymbol{v}}_1(\xi^\alpha, t) = \frac{\partial}{\partial t}\hat{\boldsymbol{n}}(\xi^\alpha, t)\bigg|_{\xi^\gamma} \ . \tag{5}$$

To find a suitable choice for the position vector in the Eulerian parametrization, we first recognize that it should represent the same body $\mathcal{M}$ as the position vector in the Lagrangian parametrization, i.e.

$$\mathcal{M} = \Big\{\hat{\boldsymbol{x}}\big(\xi^i, t\big) : \big(\xi^1, \xi^2, \xi^3\big) \in \hat{\Omega} \times \hat{\Xi}\Big\} \tag{6}$$

$$= \Big\{\boldsymbol{x}\big(\theta^i, t\big) : \big(\theta^1, \theta^2, \theta^3\big) \in \Omega \times \Xi\Big\} \ , \tag{7}$$

where $\hat{\Omega}$ and $\hat{\Xi}$, and $\Omega$ and $\Xi$ are the parametric domains associated with $\xi^\alpha$ and $\xi^3$, and $\theta^\alpha$ and $\theta^3$, respectively. Equation (7) implies that any sufficiently smooth function that maps $\Omega \times \Xi$ onto the body $\mathcal{M}$ can be used as the position vector in the Eulerian description. A suitable choice is to express the position vector as

$$\boldsymbol{x}\big(\theta^i, t\big) = \boldsymbol{x}_0(\theta^\alpha, t) + \boldsymbol{n}(\theta^\alpha, t)\, \theta^3 \ , \tag{8}$$

which coincides with the functional form of the position vector in the Lagrangian description in Eq. (1). This is particularly convenient as it implies that other kinematic quantities such as the basis vectors $\boldsymbol{g}_i$ also possess identical functional forms in the Eulerian and Lagrangian parametrizations.

The velocity vector in the Eulerian parametrization can now be obtained by taking the material time derivative of the position vector $\boldsymbol{x}\big(\theta^i, t\big)$,

$$\boldsymbol{v}\big(\theta^i, t\big) = \frac{\mathrm{d}}{\mathrm{d}t}\boldsymbol{x}\big(\theta^i, t\big) \tag{9}$$

$$= \frac{\partial}{\partial t}\boldsymbol{x}\big(\theta^i, t\big)\bigg|_{\theta^j} + \frac{\partial}{\partial \theta^k}\boldsymbol{x}\big(\theta^i, t\big)\bigg|_t \frac{\partial \theta^k}{\partial t}\bigg|_{\xi^j} \ . \tag{10}$$

However, since the parametrizations $\{\xi^i\}_{i=1,2,3}$ and $\{\theta^i\}_{i=1,2,3}$ map onto the same body, the Lagrangian parametrization can be expressed as a function of the Eulerian parametrization and vice versa, i.e.

$$\xi^i = \xi^i\big(\theta^j, t\big) \ , \tag{11}$$

$$\theta^i = \theta^i\big(\xi^j, t\big) \ , \tag{12}$$

implying that the Eulerian velocity vector must also satisfy

$$\hat{\boldsymbol{v}}\big(\xi^i, t\big) = \hat{\boldsymbol{v}}\big(\xi^i\big(\theta^j, t\big), t\big) = \boldsymbol{v}\big(\theta^j\big(\xi^i, t\big), t\big) \ . \tag{13}$$

In the following, we show that the assumptions

$$\theta^\alpha = \theta^\alpha\left(\xi^\beta, t\right) \ , \tag{14}$$

$$\dot{\theta}^3 = 0 \ , \tag{15}$$

allow us to to satisfy Eq. (13). To that end, we make the convenient, but not necessary choice,

$$\theta^3 = \theta^3\big(\xi^3\big) = \xi^3 \ , \tag{16}$$

which is also consistent with Eq. (15).

To show that the choices in Eqs. (14) and (16) are compatible with K-L kinematics, we now substitute Eq. (8) into Eq. (10) to find

$$\boldsymbol{v}\big(\theta^i, t\big) = \frac{\partial}{\partial t}\boldsymbol{x}_0(\theta^\alpha, t)\bigg|_{\theta^\beta} + \boldsymbol{a}_\gamma(\theta^\alpha, t)\ \frac{\partial \theta^\gamma}{\partial t}\bigg|_{\xi^j} + \left(\frac{\partial}{\partial t}\boldsymbol{n}(\theta^\alpha, t)\bigg|_{\theta^\beta} + \frac{\partial}{\partial \theta^\gamma}\boldsymbol{n}(\theta^\alpha, t)\bigg|_t \ \frac{\partial \theta^\gamma}{\partial t}\bigg|_{\xi^j}\right)\theta^3 + \boldsymbol{n}(\theta^\alpha, t)\dot{\theta}^3 \ . \tag{17}$$

In Eq. (17), we find the terms highlighted in green are constant through the thickness when using Eq. (14) and are therefore consistent with the result that the velocity can be at most linear through the thickness under the assumption of K-L kinematics. According to the Weingarten formula, $\boldsymbol{n}_{,\alpha} = -b_\alpha^\beta \boldsymbol{a}_\beta$, the terms highlighted in orange only have components along the in-plane directions, which could vary arbitrarily along $\theta^3$. However, when we apply the assumption in Eq. (14), $\frac{\partial \theta^\gamma}{\partial t}\big|_{\xi^j}$ is independent of $\xi^3$ and we obtain at most linear in-plane velocities through the thickness as required by the K-L assumptions. Finally, the term highlighted in blue vanishes under the assumption in Eq. (15), thus ensuring at most constant normal velocities through the thickness. Therefore, we find that the assumptions in Eqs. (14) and (16) yield the same polynomial order of the velocity components as K-L kinematics.

However, to ensure compatibility of the velocity vector in the Eulerian parametrization with the K-L assumptions, we further require, analogously to Eq. (13),

$$\hat{\boldsymbol{v}}_0(\xi^\alpha, t) = \boldsymbol{v}_0\Big(\theta^\beta(\xi^\alpha, t), t\Big) \ , \tag{18}$$

$$\hat{\boldsymbol{v}}_1(\xi^\alpha, t) = \boldsymbol{v}_1\Big(\theta^\beta(\xi^\alpha, t), t\Big) \ . \tag{19}$$

Under the assumptions in Eqs. (14) and (15), we identify from Eq. (17)

$$\boldsymbol{v}_0(\theta^\alpha,t) = \frac{\mathrm{d}}{\mathrm{d}t}\boldsymbol{x}_0(\theta^\alpha,t) \ , \tag{20}$$

$$\boldsymbol{v}_1(\theta^\alpha,t) = \frac{\mathrm{d}}{\mathrm{d}t}\boldsymbol{n}(\theta^\alpha,t) \ . \tag{21}$$

By definition of the material derivative, i.e. $\frac{\mathrm{d}}{\mathrm{d}t}\boldsymbol{x}_0(\theta^\alpha,t) = \frac{\partial}{\partial t}\boldsymbol{x}_0(\theta^\alpha,t)\big|_{\xi^i}$ and $\frac{\mathrm{d}}{\mathrm{d}t}\boldsymbol{n}(\theta^\alpha,t) = \frac{\partial}{\partial t}\boldsymbol{n}(\theta^\alpha,t)\big|_{\xi^i}$, Eqs. (20) and (21) are consistent with Eqs. (18) and (19), and consequently with K-L kinematics. Hence, we can now write the velocity in the Eulerian parametrization as

$$\boldsymbol{v}\big(\theta^i,t\big) = \boldsymbol{v}_0(\theta^\alpha,t) + \boldsymbol{v}_1(\theta^\alpha,t)\theta^3 \ , \tag{22}$$

where $\boldsymbol{v}_0(\theta^\alpha,t)$ and $\boldsymbol{v}_1(\theta^\alpha,t)$ are given in Eq. (20) and (21), respectively. Finally, the expression for the first-order velocity can be expanded further by using $\dot{\boldsymbol{n}}\cdot\boldsymbol{n}=0$ and $\dot{\boldsymbol{n}}\cdot\boldsymbol{a}_\alpha = -\boldsymbol{n}\cdot\boldsymbol{v}_{0,\alpha}$ to yield

$$\dot{\boldsymbol{n}} = v_1^\alpha \boldsymbol{a}_\alpha \tag{23}$$

$$= -\left(v^3_{0,\beta} + v_0^\lambda b_{\lambda\beta}\right) a^{\alpha\beta}\boldsymbol{a}_\alpha \ . \tag{24}$$

## 1.2 On the Eulerian Parametrization of the Mid-Surface

In Sec. 2.1 of the main text, we *chose* the normal component of the mid-surface velocity to be given by

$$v_0^3\,\boldsymbol{n} = \frac{\partial \boldsymbol{x}_0(\theta^\alpha,t)}{\partial t}\bigg|_{\theta^\beta} \ . \tag{25}$$

When we express the mid-surface velocity as the material time derivative of the mid-surface position vector $\boldsymbol{x}_0$, i.e.

$$\boldsymbol{v}_0 = \frac{\mathrm{d}\boldsymbol{x}_0}{\mathrm{d}t} = \frac{\partial \boldsymbol{x}_0}{\partial t}\bigg|_{\theta^\mu} + \frac{\partial\theta^\alpha}{\partial t}\bigg|_{\xi^\mu}\boldsymbol{a}_\alpha \tag{26}$$

$$= (\boldsymbol{v}_0\cdot\boldsymbol{n})\,\boldsymbol{n} + \frac{\partial\theta^\alpha}{\partial t}\bigg|_{\xi^\mu}\boldsymbol{a}_\alpha \ , \tag{27}$$

we find that Eq. (25) implies that the in-plane velocity of the mid-surface is related to the mid-surface parametrization by

$$v_0^\alpha = \frac{\partial\theta^\alpha}{\partial t}\bigg|_{\xi^\mu} \ . \tag{28}$$

In the following, we seek to motivate the choice in Eq. (25) for lipid membranes.

First consider the Lagrangian parametrization $\{\xi^\alpha\}_{\alpha=1,2}$ and a fixed point in parametric space $\big(\bar{\xi}^1,\bar{\xi}^2\big)$. The material point associated with $\big(\bar{\xi}^1,\bar{\xi}^2\big)$ is located on the mid-surface at $\hat{\boldsymbol{x}}_0\big(\bar{\xi}^\alpha,t\big)$ at time $t$ and at $\hat{\boldsymbol{x}}_0\big(\bar{\xi}^\alpha,t+\mathrm{d}t\big)$ at time $t+\mathrm{d}t$. The two positions of the material point are related by the mid-surface velocity $\hat{\boldsymbol{v}}_0\big(\bar{\xi}^\alpha,t\big)$, i.e.

$$\hat{\boldsymbol{x}}_0\big(\bar{\xi}^\alpha,t+\mathrm{d}t\big) = \hat{\boldsymbol{x}}_0\big(\bar{\xi}^\alpha,t\big) + \hat{\boldsymbol{v}}_0\big(\bar{\xi}^\alpha,t\big)\mathrm{d}t \ . \tag{29}$$

This statement is equivalent to the definition of the mid-surface velocity as $\hat{\boldsymbol{v}}_0 = \partial\hat{\boldsymbol{x}}_0/\partial t\big|_{\bar{\xi}^\alpha}$ and corroborates our understanding that the Lagrangian parametrization tracks material points in time.

However, the in-plane fluidity of lipid membranes can lead to significant in-plane flows, making tracking of material points with a Lagrangian parametrization challenging. Instead, we require a parametrization akin to the Eulerian parametrizations commonly used to resolve fluid flows. To show that the Eulerian parametrization $\{\theta^\alpha\}_{\alpha=1,2}$, satisfying Eqs. (25) and (28), is suitable to describe in-plane flows, consider a fixed point $\big(\bar{\theta}^1, \bar{\theta}^2\big)$ in parametric space. In contrast to the Lagrangian parametrization, an Eulerian parametrization should not track material points. This motivates the choice that the position vector $\boldsymbol{x}_0\big(\bar{\theta}^\alpha, t\big)$ on a non-deforming mid-surface with in-plane flows remains constant over time. However, when the mid-surface moves along its normal direction with velocity $v_0^3\big(\bar{\theta}^\alpha, t\big) = \boldsymbol{v}_0\big(\bar{\theta}^\alpha, t\big) \cdot \boldsymbol{n}\big(\bar{\theta}^\alpha, t\big)$, the mid-surface position vector $\boldsymbol{x}_0\big(\bar{\theta}^\alpha, t\big)$ in the Eulerian parametrization should satisfy

$$\boldsymbol{x}_0\big(\bar{\theta}^\alpha, t + \mathrm{d}t\big) = \boldsymbol{x}_0\big(\bar{\theta}^\alpha, t\big) + v_0^3\big(\bar{\theta}^\alpha, t\big)\boldsymbol{n}\big(\bar{\theta}^\alpha, t\big)\mathrm{d}t \;, \tag{30}$$

implying that in the absence of any normal velocity, $\big(\bar{\theta}^1, \bar{\theta}^2\big)$ corresponds to a fixed point on the mid-surface rather than a fixed material point. This aligns with the usual Eulerian perspective for three-dimensional fluids. Equation (30) further shows that the position vector is only displaced when there is a non-zero normal velocity. Consequently, the parametrization $\{\theta^\alpha\}_{\alpha=1,2}$ is in-plane Eulerian but out-of-plane Lagrangian, making it a suitable choice to describe the in-plane fluid and out-of-plane elastic behavior of lipid membranes. For the sake of brevity, however, we refer to $\{\theta^\alpha\}_{\alpha=1,2}$ as an Eulerian parameterization. Finally, we note that Eq. (30) is equivalent to Eq. (25) and, consequently, Eq. (28), thus justifying them as a suitable choice for lipid membranes.

## 2 Polynomial Expansions of the Christoffel Symbols

Application of the dimension reduction method proposed in [1] requires the evaluation of integral inner products of the balance laws with Chebyshev polynomials. Evaluation of these integrals becomes challenging when the balance laws contain rational polynomials. To overcome this challenge, an effective approach is to expand the rational polynomials as a series. As discussed in the main text, the contravariant basis vectors are rational polynomials and consequently, the Christoffel symbols required to evaluate partial derivatives of vectors and tensors are also rational. Therefore, we derive series expansions of the in-plane, contravariant basis vectors and the Christoffel symbols required for the divergence operator, thus facilitating the evaluation of integral inner products.

We note that in part 1 [1], it was sufficient to use truncated expansions rather than the full series expansions. However, the derivation of the $(2 + \delta)$-dimensional linear momentum balance requires series expansions to systematically eliminate higher-order stress vector coefficients arising from the stress divergence. Furthermore, when deriving the $(2 + \delta)$-dimensional angular momentum balance, series expansions are required for consistency with its three-dimensional counterpart.

### 2.1 Contravariant Basis Vectors

In this section, we derive the series expansion for the contravariant basis vectors $\boldsymbol{g}^\alpha$, with similar derivations also presented in Refs. [2, 3]. We begin by recalling the expression for the in-plane

covariant basis vectors associated with the form of the position vector in Eq. (8) (also see Sec. 2.1 of the main text),

$$\boldsymbol{g}_\alpha = \boldsymbol{a}_\alpha + \boldsymbol{n}_{,\alpha}\theta^3 \tag{31}$$

$$= \boldsymbol{a}_\alpha - b^\beta_\alpha \boldsymbol{a}_\beta\,\theta^3 \ , \tag{32}$$

where we used $\boldsymbol{n}_{,\alpha} = -b^\beta_\alpha \boldsymbol{a}_\beta$. Equation (32) can be written in tensor notation as

$$\boldsymbol{g}_\alpha = \left(\boldsymbol{i} - \boldsymbol{b}\theta^3\right) \boldsymbol{a}_\alpha, \tag{33}$$

where $\boldsymbol{b} = b^\alpha_\beta\, \boldsymbol{a}_\alpha \otimes \boldsymbol{a}^\beta$ and $\boldsymbol{i} = \boldsymbol{a}_\alpha \otimes \boldsymbol{a}^\alpha$ are the curvature and metric tensors, respectively. We now assume that the contravariant basis vectors are related to the contravariant mid-surface basis vectors through some tensor $\boldsymbol{A} = A^{\alpha\beta}\, \boldsymbol{a}_\alpha \otimes \boldsymbol{a}_\beta$, analogously to Eq. (33), i.e.

$$\boldsymbol{g}^\alpha = \boldsymbol{A}\boldsymbol{a}^\alpha \ . \tag{34}$$

To obtain an expression for $\boldsymbol{A}$, note that $\{\boldsymbol{g}_\alpha\}_{\alpha=1,2}$ and $\{\boldsymbol{a}_\alpha\}_{\alpha=1,2}$ span the same tangent space, implying the metric tensor satisfies $\boldsymbol{i} = \boldsymbol{a}_\alpha \otimes \boldsymbol{a}^\alpha = \boldsymbol{g}_\alpha \otimes \boldsymbol{g}^\alpha$. By using Eqs. (33) and (34), we thus find

$$\boldsymbol{i} = \boldsymbol{g}_\alpha \otimes \boldsymbol{g}^\alpha = \left(\boldsymbol{i} - \boldsymbol{b}\theta^3\right) \left(\boldsymbol{a}_\alpha \otimes \boldsymbol{a}^\alpha\right) \boldsymbol{A}^T \tag{35}$$

$$= \left(\boldsymbol{i} - \boldsymbol{b}\theta^3\right) \boldsymbol{A}^T \tag{36}$$

By assumption, $\theta^3 \in (-\delta/2, \delta/2)$ and $\delta\kappa_\alpha < 1$, showing that $\boldsymbol{i} - \boldsymbol{b}\theta^3$ is invertible. Therefore, $\boldsymbol{A}$ be given by

$$\boldsymbol{A} = \left(\boldsymbol{i} - \boldsymbol{b}\theta^3\right)^{-1} \ . \tag{37}$$

To invert $\boldsymbol{i} - \boldsymbol{b}\theta^3$, we start from the relation,

$$\left(\boldsymbol{i} - \boldsymbol{b}\theta^3\right) \sum_{m=0}^{N} \left(\boldsymbol{b}\theta^3\right)^m = \boldsymbol{i} - \left(\boldsymbol{b}\theta^3\right)^{N+1} \ , \tag{38}$$

which can also be written as

$$\sum_{m=0}^{N} \left(\boldsymbol{b}\theta^3\right)^m = \left(\boldsymbol{i} - \boldsymbol{b}\theta^3\right)^{-1} \left(\boldsymbol{i} - \left(\boldsymbol{b}\theta^3\right)^{N+1}\right) \ . \tag{39}$$

Using the spectral expansion of the curvature tensor $\boldsymbol{b} = \sum_{\alpha=1}^{2} \kappa_\alpha \boldsymbol{l}_\alpha \otimes \boldsymbol{l}^\alpha$ with $\boldsymbol{\kappa}_\alpha$ and $\boldsymbol{l}_\alpha = \boldsymbol{l}^\alpha$ denoting the principal curvatures and orthonormal eigenvectors, respectively, the tensor powers in Eq. (39) can be expressed as

$$\left(\boldsymbol{b}\theta^3\right)^N = \sum_{\alpha=1}^{2} \left(\kappa_\alpha\theta^3\right)^N \boldsymbol{l}_\alpha \otimes \boldsymbol{l}^\alpha \ . \tag{40}$$

From $\theta^3 \in (-\delta/2, \delta/2)$ and $\delta\kappa_\alpha < 1$, we thus obtain

$$\lim_{N\to\infty} \left(\boldsymbol{b}\theta^3\right)^N = \boldsymbol{0} \ . \tag{41}$$

Considering the limit $N \to \infty$ in Eq. (39) therefore yields the series expansion of $\left(\boldsymbol{i} - \boldsymbol{b}\theta^3\right)^{-1}$ as

$$\boldsymbol{A} = \left(\boldsymbol{i} - \boldsymbol{b}\theta^3\right)^{-1} = \sum_{m=0}^{\infty} \left(\boldsymbol{b}\theta^3\right)^m \ . \tag{42}$$

Finally, substituting Eq. (42) into Eq. (34) yields the expansion of the contravariant basis vectors,

$$\boldsymbol{g}^\alpha = \sum_{m=0}^{\infty} \boldsymbol{a}^\alpha \cdot \boldsymbol{b}^m \left(\theta^3\right)^m \tag{43}$$

$$= \sum_{m=0}^{\infty} \frac{1}{2^m} \boldsymbol{a}^\alpha \cdot \tilde{\boldsymbol{b}}^m \Theta^m \ , \tag{44}$$

where we used the symmetry of the curvature tensor and $\theta^3 = \frac{\delta}{2}\Theta$, and defined

$$\tilde{\boldsymbol{b}} = \delta \boldsymbol{b} \ . \tag{45}$$

To rewrite the series expansion in Eq. (44) in terms of Chebyshev polynomials, we expand the monomials $\Theta^m$, $m \geq 0$, as [4]

$$\Theta^m = \sum_{k=0}^{m} c_k \alpha_{mk} P_k(\Theta) \ , \tag{46}$$

where

$$c_k = \begin{cases} 1/2 \ , & \text{if } k = 0 \ , \\ 1 \ , & \text{otherwise} \ , \end{cases} \tag{47}$$

and

$$\alpha_{mk} = \begin{cases} 0 \ , & \text{if } m - k \text{ odd} \ , \\ 2^{1-m}\binom{m}{(m-k)/2} \ , & \text{if } m - k \text{ even} \ . \end{cases} \tag{48}$$

Substituting Eq. (46) into Eq. (44), we finally find the series expansion of $\boldsymbol{g}^\alpha$ in terms of Chebyshev polynomials as

$$\boldsymbol{g}^\alpha = \sum_{m=0}^{\infty} \frac{1}{2^m} \boldsymbol{a}^\alpha \cdot \tilde{\boldsymbol{b}}^m \sum_{k=0}^{m} c_k \alpha_{mk} P_k(\Theta) \ . \tag{49}$$

## 2.2 Christoffel Symbols

The three-dimensional Christoffel symbols arising from the stress vector divergence $\boldsymbol{T}^i|_i$, appearing in the linear momentum balance, are of the form $\Gamma^j_{ij}$, which can be further categorized as

$$\Gamma^\beta_{\alpha\beta} = \boldsymbol{g}_{\alpha,\beta} \cdot \boldsymbol{g}^\beta \ , \tag{50}$$

$$\Gamma^\alpha_{3\alpha} = \Gamma^\alpha_{\alpha 3} = \boldsymbol{n}_{,\alpha} \cdot \boldsymbol{g}^\alpha \ , \tag{51}$$

$$\Gamma^3_{33} = 0 \ , \tag{52}$$

$$\Gamma^3_{\alpha 3} = 0 \ , \tag{53}$$

where we used $\boldsymbol{n}_{,3} = \boldsymbol{0}$ and $\boldsymbol{n}_{,\alpha} \cdot \boldsymbol{n} = 0$. To derive a series expansion of $\Gamma^\beta_{\alpha\beta}$, we substitute the expression for the co- and contravariant basis vectors in Eqs. (31) and (44) into Eq. (50) and use $\theta^3 = \frac{\delta}{2}\Theta$ to obtain

$$\Gamma^\beta_{\alpha\beta} = \left(\boldsymbol{a}_{\alpha,\beta} + \frac{\delta}{2}\boldsymbol{n}_{,\alpha\beta}\Theta\right) \cdot \left(\sum_{m=0}^{\infty} \frac{1}{2^m}\boldsymbol{a}^\beta \cdot \tilde{\boldsymbol{b}}^m \Theta^m\right) \ . \tag{54}$$

To evaluate the term $\boldsymbol{n}_{,\alpha\beta}$, we use the relations

$$\boldsymbol{n}_{,\alpha} = -b^\beta_\alpha \boldsymbol{a}_\beta \ , \tag{55}$$

$${}^0\Gamma^\delta_{\alpha\beta} = \boldsymbol{a}_{\alpha,\beta} \cdot \boldsymbol{a}^\delta \tag{56}$$

$$\boldsymbol{a}_{\alpha,\beta} = {}^0\Gamma^\delta_{\alpha\beta}\boldsymbol{a}_\delta + b_{\alpha\beta}\boldsymbol{n} \ , \tag{57}$$

$$b^\gamma_{\alpha;\beta} = b^\gamma_{\alpha,\beta} + b^\delta_\alpha \, {}^0\Gamma^\gamma_{\delta\beta} - b^\gamma_\delta \, {}^0\Gamma^\delta_{\alpha\beta} \ , \tag{58}$$

where Eq. (55) is the Weingarten formula and ${}^0\Gamma^\delta_{\alpha\beta}$ is the mid-surface Christoffel symbol of the second kind. From Eqs. (55)–(58), we then find

$$\boldsymbol{n}_{,\alpha\beta} = -\left(b^\gamma_{\alpha;\beta}\boldsymbol{a}_\gamma + b^\gamma_\delta \, {}^0\Gamma^\delta_{\alpha\beta}\boldsymbol{a}_\gamma + b^\delta_\alpha b_{\delta\beta}\boldsymbol{n}\right) \ . \tag{59}$$

Substituting Eq, (59) into Eq. (54) and again using Eq. (56) yields the series expansion of the Christoffel symbol $\Gamma^\beta_{\alpha\beta}$,

$$\Gamma^\beta_{\alpha\beta} = {}^0\Gamma^\beta_{\alpha\beta} - \frac{1}{2}\sum_{m=0}^{\infty} \frac{1}{2^m}\boldsymbol{a}^\beta \cdot \tilde{\boldsymbol{b}}^m \boldsymbol{a}_\gamma \, \tilde{b}^\gamma_{\alpha;\beta}\Theta^{m+1} \ . \tag{60}$$

Equation (60) can be expressed in terms of Chebsyhsev polynomials by using Eq. (46), resulting in

$$\Gamma^\beta_{\alpha\beta} = {}^0\Gamma^\beta_{\alpha\beta} - \frac{1}{2}\sum_{m=0}^{\infty} \frac{1}{2^m}\boldsymbol{a}^\beta \cdot \tilde{\boldsymbol{b}}^m \boldsymbol{a}_\gamma \, \tilde{b}^\gamma_{\alpha;\beta}\left(\sum_{k=0}^{m+1} c_k \alpha_{(m+1)k} P_k(\Theta)\right) \ . \tag{61}$$

To find an expression for the Christoffel symbol in Eq. (51), we substitute Eqs. (44) and (55), leading to

$$\delta\Gamma^\alpha_{3\alpha} = -\tilde{b}^\beta_\alpha \boldsymbol{a}_\beta \cdot \left(\sum_{m=0}^{\infty} \frac{1}{2^m}\boldsymbol{a}^\alpha \cdot \tilde{\boldsymbol{b}}^m \Theta^m\right) \tag{62}$$

$$= -\sum_{m=0}^{\infty} \frac{1}{2^m}\boldsymbol{a}^\alpha \cdot \tilde{\boldsymbol{b}}^{m+1}\boldsymbol{a}_\alpha \Theta^m \tag{63}$$

$$= -\sum_{m=0}^{\infty} \frac{1}{2^m} \operatorname{tr}\left(\tilde{\boldsymbol{b}}^{m+1}\right)\Theta^m \tag{64}$$

$$= -\sum_{m=0}^{\infty} \frac{1}{2^m} \operatorname{tr}\left(\tilde{\boldsymbol{b}}^{m+1}\right)\left(\sum_{k=0}^{m+1} c_k \alpha_{mk} P_k(\Theta)\right) \ . \tag{65}$$

# 3 Reactive Stresses

In Sec. 2.2 of the main text, we introduced the interpretation of K-L kinematics as kinematic constraints that are enforced through reactive stresses. In this section, we first show that the constraints can be equivalently formulated in terms of the metric tensor. Furthermore, we examine these constraints within the framework of hyperelastic materials, where the equations of motion can be derived from a minimization problem. In that case, the reactive stresses are Lagrange multipliers that enforce the K-L constraints. We can relax these constraints by invoking the penalty method, which converges to the method of Lagrange multipliers for large penalty parameters. By employing the penalty approach, we gain insight into the conditions under which the reactive stresses can be truncated at first order.

## 3.1 Kirchhoff-Love Kinematics as a Constraint

In Sec. 2.2 of the main text, we discussed that, under the assumption of K-L kinematics, the metric tensor takes the form

$$\hat{g}_{ij} = \hat{\boldsymbol{g}}_i \cdot \hat{\boldsymbol{g}}_j = \begin{bmatrix} [\hat{g}_{\alpha\beta}] & \boldsymbol{0} \\ \boldsymbol{0} & 1 \end{bmatrix}_{ij} \ , \tag{66}$$

or, equivalently,

$$\hat{g}_{\alpha 3} = \hat{g}_{3\alpha} = 0 \ , \tag{67}$$

$$\hat{g}_{33} = 1 \ . \tag{68}$$

In this section, we show that Eqs. (67) and (68) are satisfied if and only if the K-L assumptions in Eq. (1) are satisfied. Therefore, K-L kinematics can be formulated as a set of constraints on the metric tensor. To show this, consider a general position vector of a point $\hat{\boldsymbol{x}}' \in \mathcal{M}$ in the Lagrangian description. Such a general position vector can be written as a series expansion of the form

$$\hat{\boldsymbol{x}}'\left(\xi^i, t\right) = \sum_{k=0}^{\infty} \hat{\boldsymbol{x}}'_k(\xi^\alpha, t) \left(\xi^3\right)^k \ . \tag{69}$$

From this, we find the covariant basis vectors

$$\hat{\boldsymbol{g}}'_\alpha = \sum_{k=0}^{\infty} \hat{\boldsymbol{x}}'_{k,\alpha} \left(\xi^3\right)^k \ , \tag{70}$$

$$\hat{\boldsymbol{g}}'_3 = \sum_{k=0}^{\infty} \hat{\boldsymbol{x}}'_{k+1} \left(k+1\right) \left(\xi^3\right)^k \ , \tag{71}$$

and taking the appropriate dot products yields

$$\hat{g}'_{3\alpha} = \hat{g}'_{\alpha 3} = \sum_{k=0}^{\infty} \left( \sum_{l=0}^{k} \hat{\boldsymbol{x}}'_{l,\alpha} \cdot \hat{\boldsymbol{x}}'_{k-l+1} \left(k-l+1\right) \right) \left(\xi^3\right)^k \ , \tag{72}$$

$$\hat{g}'_{33} = \sum_{k=0}^{\infty} \left( \sum_{l=0}^{k} \hat{\boldsymbol{x}}'_{l+1} \cdot \hat{\boldsymbol{x}}'_{k-l+1} \left(l+1\right) \left(k-l+1\right) \right) \left(\xi^3\right)^k \ . \tag{73}$$

Using the expansions in Eqs. (69), (72), and (73), we can show that Eqs. (67) and (68) are not only necessary but also sufficient conditions to satisfy K-L kinematics. To this end, we observe that Eqs. (72) and (73) imply that for $\hat{g}'_{ij}$ to satisfy Eqs. (67) and (68), we require

$$\sum_{l=0}^{k} \hat{\boldsymbol{x}}'_{l,\alpha} \cdot \hat{\boldsymbol{x}}'_{k-l+1} \, (k-l+1) = 0 \ , \quad \forall k \in \mathbb{N}_0 \ , \tag{74}$$

$$\hat{\boldsymbol{x}}'_1 \cdot \hat{\boldsymbol{x}}'_1 = 1 \ , \tag{75}$$

$$\sum_{l=0}^{k} \hat{\boldsymbol{x}}'_{l+1} \cdot \hat{\boldsymbol{x}}'_{k-l+1} \, (l+1) \, (k-l+1) = 0 \ , \quad \forall k \in \mathbb{N} \ . \tag{76}$$

For the remainder of the derivation, it is convenient to rewrite Eqs. (74) and (76) as

$$\hat{\boldsymbol{x}}'_{0,\alpha} \cdot \hat{\boldsymbol{x}}'_{k+1} \, (k+1) + \sum_{l=1}^{k} \hat{\boldsymbol{x}}'_{l,\alpha} \cdot \hat{\boldsymbol{x}}'_{k-l+1} \, (k-l+1) = 0 \ , \quad \forall k \in \mathbb{N}_0 \ , \tag{77}$$

$$2\hat{\boldsymbol{x}}'_1 \cdot \hat{\boldsymbol{x}}'_{k+1} \, (k+1) + \sum_{l=1}^{k-1} \hat{\boldsymbol{x}}'_{l+1} \cdot \hat{\boldsymbol{x}}'_{k-l+1} \, (l+1) \, (k-l+1) = 0 \ , \quad \forall k \in \mathbb{N} \ . \tag{78}$$

Considering the case $k = 0$ in Eq. (77) then yields

$$\hat{\boldsymbol{x}}'_{0,\alpha} \cdot \hat{\boldsymbol{x}}'_1 = 0 \ , \tag{79}$$

implying that $\hat{\boldsymbol{x}}'_{0,\alpha}$ is orthogonal to $\hat{\boldsymbol{x}}'_1$. This shows that the set $\{\hat{\boldsymbol{x}}'_{0,1}, \hat{\boldsymbol{x}}'_{0,2}, \hat{\boldsymbol{x}}'_1\}$ forms a basis of $\mathbb{R}^3$ at every point in $\mathcal{M}$ if $\xi^1$ and $\xi^2$ are not collinear. Therefore, if

$$\hat{\boldsymbol{x}}'_i = \mathbf{0}, \quad 2 \le i \le k \ , \tag{80}$$

Eqs. (77) and (78) imply, respectively,

$$\hat{\boldsymbol{x}}'_{0,\alpha} \cdot \hat{\boldsymbol{x}}'_{k+1} = 0 \ , \tag{81}$$

$$\hat{\boldsymbol{x}}'_1 \cdot \hat{\boldsymbol{x}}'_{k+1} = 0 \ . \tag{82}$$

However, since $\{\hat{\boldsymbol{x}}'_{0,1}, \hat{\boldsymbol{x}}'_{0,2}, \hat{\boldsymbol{x}}'_1\}$ forms a basis of $\mathbb{R}^3$, Eqs. (81) and (82) imply that $\hat{\boldsymbol{x}}'_{k+1} = \mathbf{0}$. Finally, when we consider the case $k = 1$ in Eqs. (77) and (78), we find, upon using Eq. (75),

$$\hat{\boldsymbol{x}}'_2 = \mathbf{0} \ . \tag{83}$$

Equations (80)–(83) therefore show that $\hat{\boldsymbol{x}}'_k = \mathbf{0}$, $\forall k \ge 2$, demonstrating that all higher-order position vector coefficients vanish if Eqs. (67) and (68) are satisfied, i.e.

$$\hat{g}'_{33} = 1 \quad \text{and} \quad \hat{g}'_{\alpha 3} = \hat{g}'_{3\alpha} = 0 \quad \Longleftrightarrow \quad \hat{\boldsymbol{x}}'_k = \mathbf{0}, \quad \forall k \ge 2 \ . \tag{84}$$

This reduces the position vector in Eq. (69) to

$$\hat{\boldsymbol{x}}'(\xi^i, t) = \hat{\boldsymbol{x}}'_0(\xi^\alpha, t) + \hat{\boldsymbol{x}}'_1(\xi^\alpha, t)\xi^3 \ . \tag{85}$$

Equation (85) shows that the zeroth-order coefficient $\hat{\boldsymbol{x}}_0'$ describes the mid-surface of the body $\mathcal{M}$, in the sense that $\hat{\boldsymbol{x}}'\left(\xi^i, t\right)$ is symmetric about $\hat{\boldsymbol{x}}_0'(\xi^\alpha, t)$ with respect to $\xi^3$. From Eqs. (75) and (79), it is apparent that $\boldsymbol{x}_1'(\xi^\alpha, t)$ is a unit vector orthogonal to the tangent vectors of the mid-surface, $\boldsymbol{x}_{0,\alpha}'(\xi^\alpha, t)$. Thus, it follows that $\boldsymbol{x}_1'(\xi^\alpha, t)$ is the normal vector to the mid-surface, i.e.

$$\hat{\boldsymbol{x}}_1'(\xi^\alpha, t) = \hat{\boldsymbol{n}}(\xi^\alpha, t) \ . \tag{86}$$

Equations (84)–(86) now show that the choice of Kirchhoff-Love kinematics is equivalent to satisfying Eqs. (67) and (68). As discussed in Sec. 2.2 of the main text, the latter conditions can be equivalently expressed as

$$\hat{\Gamma}_i(\hat{\boldsymbol{C}}) \coloneqq \hat{\boldsymbol{G}}_i \cdot \hat{\boldsymbol{E}}\hat{\boldsymbol{G}}_3 = \hat{\boldsymbol{G}}_3 \cdot \hat{\boldsymbol{E}}\hat{\boldsymbol{G}}_i = 0 \ , \tag{87}$$

where $\hat{\boldsymbol{E}}$ is the right Green-Lagrange strain tensor with respect to a reference configuration satisfying the K-L assumptions, and $\hat{\boldsymbol{G}}_i$ are the basis vectors associated with that reference configuration.

## 3.2 On the Truncation of Reactive Stresses

In Sec. 4.3 of the main text, we found that the linear momentum balance contains infinite sums of the Chebyshev coefficients of the stress vector $\boldsymbol{T}^3$. Since $\boldsymbol{T}^3$ depends only on the reactive stresses (see Sec. 4.2 of the main text), truncating these infinite sums requires knowledge of the magnitude of the expansion coefficients of the reactive stresses. These cannot be determined a-priori but must instead be solved for along with all other unknowns. However, we may obtain order of magnitude estimates by considering a case where the position vector can be determined through a constrained minimization problem. This allows us to relax the constraints imposed by the choice of K-L kinematics using the penalty method. Using this approach, we can obtain kinematic assumptions required to make order of magnitude estimates for the reactive stress coefficients, permitting the truncation of the infinite sums appearing in the linear momentum balance in Sec. 4.3 of the main text.

Before analyzing the reactive stresses, consider the following constrained minimization problem with a unique solution,

$$y^\dagger = \arg\min_y f(y) \quad \text{subject to } \gamma(y) = 0 \ , \tag{88}$$

where $\gamma(y) = 0$ is some constraint. By using the method of Lagrange multipliers, we can reframe this constrained minimization problem as an unconstrained minimization problem,

$$(y^\dagger, \lambda^\dagger) = \arg\min_{y,\,\lambda} \left(f(y) - \lambda\gamma(y)\right) \ , \tag{89}$$

where $\lambda$ is the Lagrange multiplier. Alternatively, the minimization problem in Eq. (88) can be solved by adding a quadratic penalty term, resulting in

$$y_\ell^\ddagger = \arg\min_y \left(f(y) + \frac{K_\ell}{2}\gamma(y)^2\right) \ , \tag{90}$$

where $K_\ell$ is a penalty parameter. For a sequence $\{K_\ell\}$, $0 < K_\ell < K_{\ell+1}$ that diverges to infinity, the sequence $\left\{y_\ell^\ddagger\right\}$ converges to $y^\dagger$, and the sequence $\left\{-K_\ell\,\gamma\left(y_\ell^\ddagger\right)\right\}$ converges to $\lambda^\dagger$ [5]. This result motivates the relaxation of the constraints in Eq. (87) below.

To be able to apply the aforementioned methods for constrained minimization problems, we consider a hyperelastic material[1]. In this case, it is convenient to use the Lagrangian parametrization and consider the position vector as the fundamental unknown. For hyperelastic materials, we can use the principle of virtual work to solve an elastic boundary value problem as a minimization problem of the form [6]

$$\hat{\boldsymbol{x}}^* = \arg\min_{\hat{\boldsymbol{x}}'} \left[ \int_{\mathcal{M}_0} \Pi\Big(\hat{\boldsymbol{E}}(\hat{\boldsymbol{x}}')\Big) \, \mathrm{d}V_0 \right] , \tag{91}$$

where $\Pi$ is the virtual work functional and $\hat{\boldsymbol{E}}$ is the Euler-Lagrange strain tensor defined with respect to a stationary and stress-free reference configuration $\mathcal{M}_0$. Note that in Eq. (91), minimization is performed over arbitrary position vectors $\boldsymbol{x}'$ not necessarily satisfying the K-L assumptions. Thus, to account for the K-L constraints in Eq. (87), we must consider the constrained minimization problem

$$\hat{\boldsymbol{x}}^\dagger = \arg\min_{\hat{\boldsymbol{x}}'} \left[ \int_{\mathcal{M}_0} \Pi\Big(\hat{\boldsymbol{E}}(\hat{\boldsymbol{x}}')\Big) \, \mathrm{d}V_0 \right] \quad \text{subject to } \hat{\Gamma}_i\Big(\hat{\boldsymbol{E}}(\hat{\boldsymbol{x}}')\Big) = 0 \ , \ i = 1,2,3 \ , \tag{92}$$

while additionally assuming that $\mathcal{M}_0$ satisfies the K-L assumptions. We may then define $\mathcal{M}^\dagger = \Big\{ \hat{\boldsymbol{x}}^\dagger(\xi^i, t) : (\xi^1, \xi^2, \xi^3) \in \hat{\Omega} \times \hat{\Xi} \Big\}$ as the configuration of the body associated with the solution to this constrained minimization problem.

Before relaxing the constrained problem in Eq. (92), we note that the constraints in Eq. (87) are agnostic to the choice of reference configuration as long as it satisfies the K-L assumptions. Therefore, we can formally choose $\mathcal{M}^\dagger$ as the reference configuration for the Green-Lagrange strain used in the constraints $\hat{\Gamma}_i$. This choice allows us to apply the assumption of small deformations when relaxing the constrained problem in Eq. (92). To reformulate Eq. (92) using the Green-Lagrange strain with respect to $\mathcal{M}^\dagger$, consider the generic position vector $\boldsymbol{x}'$ as the unconstrained current configuration. Then, the deformation gradient with respect to the constrained solution $\boldsymbol{x}^\dagger$ and the corresponding right Cauchy-Green tensor and Green-Lagrange strain tensor take the form

$$\hat{\boldsymbol{F}}'^\dagger(\hat{\boldsymbol{x}}') = \nabla_{\hat{\boldsymbol{x}}^\dagger} \hat{\boldsymbol{x}}' = \hat{\boldsymbol{g}}'_i \otimes \hat{\boldsymbol{g}}^{\dagger i} \ , \tag{93}$$

$$\hat{\boldsymbol{C}}'^\dagger(\hat{\boldsymbol{x}}') = \Big(\hat{\boldsymbol{F}}'^\dagger(\hat{\boldsymbol{x}}')\Big)^T \hat{\boldsymbol{F}}'^\dagger(\hat{\boldsymbol{x}}') = \hat{g}'_{ij} \, \hat{\boldsymbol{g}}^{\dagger i} \otimes \hat{\boldsymbol{g}}^{\dagger j} \ , \tag{94}$$

$$\hat{\boldsymbol{E}}'^\dagger(\hat{\boldsymbol{x}}') = \frac{1}{2}\Big(\hat{\boldsymbol{C}}'^\dagger(\hat{\boldsymbol{x}}') - \mathbf{1}\Big) = \frac{1}{2}\Big(\hat{g}'_{ij} - \hat{g}^\dagger_{ij}\Big) \hat{\boldsymbol{g}}^{\dagger i} \otimes \hat{\boldsymbol{g}}^{\dagger j} \ , \tag{95}$$

where *prime* and *dagger* symbols indicate quantities defined with respect to $\boldsymbol{x}'$ and $\boldsymbol{x}^\dagger$, respectively. With $\hat{\boldsymbol{E}}'^\dagger$ as the choice of Green-Lagrange strain in the constraints $\hat{\Gamma}_i$, the constrained problem in Eq. (92) becomes

$$\hat{\boldsymbol{x}}^\dagger = \arg\min_{\hat{\boldsymbol{x}}'} \left[ \int_{\mathcal{M}_0} \Pi\Big(\hat{\boldsymbol{E}}(\hat{\boldsymbol{x}}')\Big) \, \mathrm{d}V_0 \right] \quad \text{subject to } \hat{\Gamma}_i\Big(\hat{\boldsymbol{E}}'^\dagger(\hat{\boldsymbol{x}}')\Big) = 0 \ , \ i = 1,2,3 \ . \tag{96}$$

[1]For hyperelastic materials, the stress tensor can be expressed as the derivative of a stored energy functional $W(\hat{\boldsymbol{E}})$, i.e. $\boldsymbol{\sigma} \propto \frac{\partial W(\hat{\boldsymbol{E}})}{\partial \hat{\boldsymbol{E}}}$. Note, however, that the viscous nature of lipid membranes implies that they are *not* hyperelastic materials. In Sec. 3.3 of the main text, we discuss the applicability of the procedure presented here to other kinds of materials.

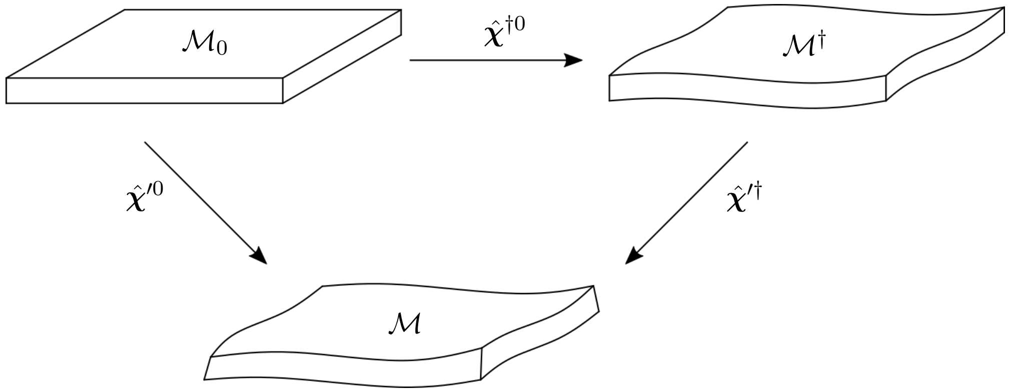


Figure 1: The current configuration $\mathcal{M}$, stress-free reference configuration $\mathcal{M}_0$, and the constrained reference configuration $\mathcal{M}^\dagger$ together with the mappings $\chi^\bullet$ between these configurations.

where the Green-Lagrange strain used in the virtual work functional remains with respect to the stress-free configuration $\mathcal{M}_0$.

We now relax the constrained minimization problem in Eq. (96) using the penalty formulation in Eq. (90). This yields the unconstrained minimization problem

$$\hat{\boldsymbol{x}}^\ddagger = \arg\min_{\hat{\boldsymbol{x}}'} \left[ \int_{\mathcal{M}_0} \Pi\Big(\hat{\boldsymbol{E}}(\hat{\boldsymbol{x}}')\Big)\, \mathrm{d}V_0 + \frac{1}{2}\sum_{i=1}^{3} K_i \int_{\mathcal{M}^\dagger} \hat{\Gamma}_i\Big(\hat{\boldsymbol{E}}'^\dagger(\hat{\boldsymbol{x}}')\Big)^2 \,\mathrm{d}V^\dagger \right] , \tag{97}$$

with $K_i$ being the penalty parameter associated with constraint $\hat{\Gamma}_i$. We note here that the penalty term is integrated over the constrained configuration $\mathcal{M}^\dagger$ instead of the stress-free configuration $\mathcal{M}_0$. To find the stresses associated with the constraints $\hat{\Gamma}_i$, we introduce the following mappings between the configurations $\mathcal{M}_0$, $\mathcal{M}^\dagger$, and $\mathcal{M}$:

$$\hat{\boldsymbol{\chi}}^{\dagger 0} : \mathcal{M}_0 \to \mathcal{M}^\dagger , \tag{98}$$

$$\hat{\boldsymbol{\chi}}'^{\dagger} : \mathcal{M}^\dagger \to \mathcal{M} , \tag{99}$$

$$\hat{\boldsymbol{\chi}}'^{0} : \mathcal{M}_0 \to \mathcal{M} , \tag{100}$$

as illustrated in Fig. 1. These three mappings are respectively associated with the deformation gradients

$$\hat{\boldsymbol{F}}^{\dagger 0} = \nabla \hat{\boldsymbol{\chi}}^{\dagger 0} , \tag{101}$$

$$\hat{\boldsymbol{F}}'^{\dagger} = \nabla \hat{\boldsymbol{\chi}}'^{\dagger} , \tag{102}$$

$$\hat{\boldsymbol{F}} = \nabla \hat{\boldsymbol{\chi}}'^{0} , \tag{103}$$

with determinants $\hat{J}^{\dagger 0} = \det \hat{\boldsymbol{F}}^{\dagger 0}$, $\hat{J}'^{\dagger} = \det \hat{\boldsymbol{F}}'^{\dagger}$, and $\hat{J} = \det \hat{\boldsymbol{F}}$. Note that the deformation gradient of $\hat{\boldsymbol{\chi}}'^{\dagger}$ was already introduced in Eq. (93). However, for the following derivations, it is convenient to redefine it in terms of the mapping $\hat{\boldsymbol{\chi}}'^{\dagger}$.

The mapping $\hat{\boldsymbol{\chi}}^{\dagger 0}$ now allows us to transform the second integral in Eq. (97) into an integral over the stress-free reference configuration $\mathcal{M}_0$,

$$\hat{\boldsymbol{x}}^\ddagger = \arg\min_{\hat{\boldsymbol{x}}'} \left[ \int_{\mathcal{M}_0} \Pi\Big(\hat{\boldsymbol{E}}(\hat{\boldsymbol{x}}')\Big)\, \mathrm{d}V_0 + \int_{\mathcal{M}_0} \Pi_{\mathrm{P}}\Big(\hat{\boldsymbol{E}}'^\dagger\Big)\hat{J}^{\dagger 0}\, \mathrm{d}V_0 \right] , \tag{104}$$

where we defined the sum of the penalty terms as

$$\Pi_{\mathrm{P}}\left(\hat{\boldsymbol{E}}'^{\dagger}\right) = \frac{1}{2}\sum_{i=1}^{3} K_i \hat{\Gamma}_i\left(\hat{\boldsymbol{E}}'^{\dagger}\right)^2 . \tag{105}$$

The first Piola-Kirchhoff stress $\hat{\boldsymbol{P}}^0$ associated with the minimization problem in Eq. (104) can then be evaluated using the relation [6],

$$\hat{\boldsymbol{P}}^0 = \frac{\partial}{\partial \hat{\boldsymbol{F}}}\left(\Pi(\hat{\boldsymbol{E}}) + \hat{J}^{\dagger 0}\Pi_{\mathrm{P}}(\hat{\boldsymbol{E}}'^{\dagger})\right) . \tag{106}$$

However, the Green-Lagrange strain $\hat{\boldsymbol{E}}'^{\dagger}$ is defined with respect to the constrained configuration such that further analysis is required to evaluate the second term of Eq. (106).

To proceed, we rewrite the deformation gradient $\hat{\boldsymbol{F}}'^{\dagger}$ in terms of the deformation gradient $\hat{\boldsymbol{F}}$. To that end, we note that the mapping between $\mathcal{M}^{\dagger}$ and $\mathcal{M}$ can be expressed as

$$\hat{\boldsymbol{\chi}}'^{\dagger}(\boldsymbol{x}^{\dagger}) = \hat{\boldsymbol{\chi}}'^{0} \circ \left(\hat{\boldsymbol{\chi}}^{\dagger 0}\right)^{-1}(\boldsymbol{x}^{\dagger}) . \tag{107}$$

By taking the gradient of Eq. (107) and using Eqs. (101)–(103), we find

$$\hat{\boldsymbol{F}}'^{\dagger} = \hat{\boldsymbol{F}}\left(\hat{\boldsymbol{F}}^{\dagger 0}\right)^{-1} . \tag{108}$$

Therefore, we can use the chain rule in Eq. (106) to find

$$\hat{\boldsymbol{P}}^0 = \frac{\partial}{\partial \hat{\boldsymbol{F}}}\Pi(\hat{\boldsymbol{E}}) + \hat{J}^{\dagger 0}\left(\frac{\partial}{\partial \hat{\boldsymbol{F}}'^{\dagger}}\Pi_{\mathrm{P}}(\hat{\boldsymbol{E}}'^{\dagger})\right) : \frac{\partial \hat{\boldsymbol{F}}'^{\dagger}}{\partial \hat{\boldsymbol{F}}} , \tag{109}$$

where the *colon* symbol indicates a double contraction. By noting $\left(\hat{\boldsymbol{F}}^{\dagger 0}\right)^{-1} = \boldsymbol{G}_i \otimes \boldsymbol{g}^{\dagger i}$, we find

$$\frac{\partial \Pi_{\mathrm{P}}}{\partial \hat{\boldsymbol{F}}'^{\dagger}} : \frac{\partial \hat{\boldsymbol{F}}'^{\dagger}}{\partial \hat{\boldsymbol{F}}} = \frac{\partial \Pi_{\mathrm{P}}}{\partial \hat{\boldsymbol{F}}'^{\dagger}}\left(\hat{\boldsymbol{F}}^{\dagger 0}\right)^{-T} . \tag{110}$$

Using this result, we write the reactive stress contribution to the first Piola-Kirchhoff stress associated with the stress-free reference configuration $\mathcal{M}_0$, as

$$\hat{\boldsymbol{P}}^0_{\mathrm{r}} = \hat{J}^{\dagger 0}\frac{\partial \Pi_{\mathrm{P}}}{\partial \hat{\boldsymbol{F}}'^{\dagger}}\left(\hat{\boldsymbol{F}}^{\dagger 0}\right)^{-T} . \tag{111}$$

To be able to use the assumption of small deformations, we seek to transform $\hat{\boldsymbol{P}}^0_{\mathrm{r}}$ into a stress in the reference configuration $\mathcal{M}^{\dagger}$. To this end, we may use the Piola Transform [6] to obtain,

$$\mathrm{div}_0\left(\hat{\boldsymbol{P}}^0_r\right) = \hat{J}^{\dagger 0}\mathrm{div}_{\dagger}\left(\frac{1}{\hat{J}^{\dagger 0}}\hat{\boldsymbol{P}}^0_r\left(\hat{\boldsymbol{F}^{\dagger 0}}\right)^T\right) = \hat{J}^{\dagger 0}\mathrm{div}_{\dagger}\left(\frac{\partial \Pi_{\mathrm{P}}}{\partial \hat{\boldsymbol{F}}'^{\dagger}}\right) , \tag{112}$$

where $\mathrm{div}_0(\bullet)$ and $\mathrm{div}_{\dagger}(\bullet)$ are the divergence operators with respect to $\mathcal{M}_0$ and $\mathcal{M}^{\dagger}$, respectively. Therefore, we identify the reactive stress contribution to the first Piola-Kirchhoff stress associated with $\mathcal{M}^{\dagger}$ as

$$\hat{\boldsymbol{P}}^{\dagger}_{\mathrm{r}} = \frac{\partial \Pi_{\mathrm{P}}}{\partial \hat{\boldsymbol{F}}'^{\dagger}} . \tag{113}$$

This result can also be obtained by mapping $\hat{\boldsymbol{P}}_{\mathrm{r}}^{0}$ to the Cauchy stress and subsequently to the first Piola-Kirchhoff stress associated with $\mathcal{M}^{\dagger}$. To see this, we express the Cauchy stress as [7]

$$\hat{\boldsymbol{\sigma}}_{\mathrm{r}} = \hat{J}^{-1}\hat{\boldsymbol{P}}_{\mathrm{r}}^{0}\hat{\boldsymbol{F}}^{T} = \left(\hat{J}'^{\dagger}\right)^{-1}\hat{\boldsymbol{P}}_{\mathrm{r}}^{\dagger}\left(\hat{\boldsymbol{F}}'^{\dagger}\right)^{T} \ , \tag{114}$$

implying that the first Piola-Kirchhoff stress associated with $\mathcal{M}^{\dagger}$ is given by

$$\hat{\boldsymbol{P}}_{\mathrm{r}}^{\dagger} = \hat{J}'^{\dagger}\hat{\boldsymbol{\sigma}}_{\mathrm{r}}\left(\hat{\boldsymbol{F}}'^{\dagger}\right)^{-T} \tag{115}$$

$$= \hat{J}^{-1}\hat{J}'^{\dagger}\hat{J}^{\dagger 0}\frac{\partial \Pi_{\mathrm{P}}}{\partial \hat{\boldsymbol{F}}'^{\dagger}}\left(\hat{\boldsymbol{F}}^{\dagger 0}\right)^{-T}\hat{\boldsymbol{F}}^{T}\left(\hat{\boldsymbol{F}}'^{\dagger}\right)^{-T} \ , \tag{116}$$

where we substituted Eq. (111). From Eq. (108), we further find,

$$\hat{J}^{-1}\hat{J}'^{\dagger}\hat{J}^{\dagger 0} = 1 \ , \tag{117}$$

$$\left(\hat{\boldsymbol{F}}^{\dagger 0}\right)^{-T}\hat{\boldsymbol{F}}^{T}\left(\hat{\boldsymbol{F}}'^{\dagger}\right)^{-T} = \mathbf{1} \ , \tag{118}$$

thus confirming the result in Eq. (113).

While Eq. (113) is expressed in terms of the derivative with respect to the deformation gradient, the constraints in Eq. (87) are written in terms of the Green-Lagrange strain. Therefore, we apply the chain rule to obtain [6],

$$\hat{\boldsymbol{P}}_{\mathrm{r}}^{\dagger} = \hat{\boldsymbol{F}}'^{\dagger}\frac{\partial \Pi_{\mathrm{P}}}{\partial \hat{\boldsymbol{E}}'^{\dagger}} \tag{119}$$

Using this result, we find the corresponding second Piola-Kirchhoff stress associated with the constrained configuration $\mathcal{M}^{\dagger}$ as

$$\boldsymbol{S}_{\mathrm{r}}^{\dagger} = \frac{\partial \Pi_{\mathrm{P}}}{\partial \hat{\boldsymbol{E}}'^{\dagger}} \ , \tag{120}$$

which yields

$$\hat{\boldsymbol{S}}_{\mathrm{r}}^{\dagger} = \sum_{i=1}^{3}\hat{\boldsymbol{S}}_{\mathrm{r}i}^{\dagger} \ , \quad \text{where} \tag{121}$$

$$\hat{\boldsymbol{S}}_{\mathrm{r}i}^{\dagger} = \frac{1}{2}K_i\hat{\Gamma}_i\left(\hat{\boldsymbol{E}}'^{\dagger}\left(\boldsymbol{x}^{\ddagger}\right)\right)\left(\hat{\boldsymbol{g}}_i^{\dagger}\otimes\hat{\boldsymbol{g}}_3^{\dagger}+\hat{\boldsymbol{g}}_3^{\dagger}\otimes\hat{\boldsymbol{g}}_i^{\dagger}\right) \ . \tag{122}$$

The above discussion of the stresses associated with the constraints $\hat{\Gamma}_i$ is formulated in terms of a general current configuration $\mathcal{M}$. We now seek to analyze the stresses associated with the configuration that is the solution of the penalty-constrained problem in Eq. (97). To that end, we assume the difference between the solutions of the exact problem in Eq. (92) and the relaxed problem in Eq. (97) is small, i.e.

$$\hat{\boldsymbol{x}}^{\ddagger} = \hat{\boldsymbol{x}}^{\dagger} + \varepsilon\hat{\boldsymbol{u}}^{\ddagger} \ , \tag{123}$$

for some small parameter $\varepsilon$. This is motivated by the result that the K-L assumptions become exact for the special case of linear elastic thin plates[2] with vanishing thickness [9–14]. Using the

[2]A thin plate is a shell-like body with a flat reference configuration [8].

assumption of small deformations, the deformation gradient, right Cauchy-Green tensor, and Green-Lagrange strain can be written as

$$\hat{\boldsymbol{F}}^{\ddagger\dagger} := \hat{\boldsymbol{F}}'^{\dagger}\left(\hat{\boldsymbol{x}}^{\ddagger}\right) = \mathbf{1} + \varepsilon \underbrace{\frac{\partial \hat{\boldsymbol{u}}^{\ddagger}}{\partial \xi^{i}} \otimes \hat{\boldsymbol{g}}^{\dagger i}}_{=\hat{\boldsymbol{H}}^{\ddagger\dagger}} = \mathbf{1} + \varepsilon \hat{\boldsymbol{H}}^{\ddagger\dagger} \ , \tag{124}$$

$$\hat{\boldsymbol{C}}^{\ddagger\dagger} := \hat{\boldsymbol{C}}'^{\dagger}\left(\hat{\boldsymbol{x}}^{\ddagger}\right) = \mathbf{1} + \varepsilon \left( \left(\hat{\boldsymbol{H}}^{\ddagger\dagger}\right)^{T} + \hat{\boldsymbol{H}}^{\ddagger\dagger} \right) + \mathcal{O}\left(\varepsilon^{2}\right) \ , \tag{125}$$

$$\hat{\boldsymbol{E}}^{\ddagger\dagger} := \hat{\boldsymbol{E}}'^{\dagger}\left(\hat{\boldsymbol{x}}^{\ddagger}\right) = \frac{\varepsilon}{2} \left( \left(\hat{\boldsymbol{H}}^{\ddagger\dagger}\right)^{T} + \hat{\boldsymbol{H}}^{\ddagger\dagger} \right) + \mathcal{O}\left(\varepsilon^{2}\right) \ . \tag{126}$$

With these definitions on hand, we first evaluate the term $\hat{\Gamma}_{i}\left(\hat{\boldsymbol{E}}^{\ddagger\dagger}\right)$ in Eq. (122). To that end, we express $\hat{\boldsymbol{H}}^{\ddagger\dagger}$ as

$$\varepsilon \hat{\boldsymbol{H}}^{\ddagger\dagger} = \frac{\partial\left(\hat{\boldsymbol{x}}^{\ddagger} - \hat{\boldsymbol{x}}^{\dagger}\right)}{\partial \xi^{\alpha}} \otimes \frac{\partial \xi^{\alpha}}{\partial \hat{\boldsymbol{x}}^{\dagger}} + \frac{\partial\left(\hat{\boldsymbol{x}}^{\ddagger} - \hat{\boldsymbol{x}}^{\dagger}\right)}{\partial \xi^{3}} \otimes \frac{\partial \xi^{3}}{\partial \hat{\boldsymbol{x}}^{\dagger}} \ , \tag{127}$$

where we used $\varepsilon \boldsymbol{u}^{\ddagger} = \hat{\boldsymbol{x}}^{\ddagger} - \hat{\boldsymbol{x}}^{\dagger}$. By expanding the position vector $\hat{\boldsymbol{x}}^{\ddagger}$ in terms of Chebyshev polynomials as

$$\hat{\boldsymbol{x}}^{\ddagger} = \sum_{i=0}^{\infty} \hat{\boldsymbol{x}}_{i}^{\ddagger} P_{i}(\Theta) \ , \tag{128}$$

and using $\hat{\boldsymbol{g}}_{\alpha}^{\dagger} = \hat{\boldsymbol{g}}_{\alpha}$, $\hat{\boldsymbol{g}}^{\dagger\alpha} = \hat{\boldsymbol{g}}^{\alpha}$, and $\hat{\boldsymbol{g}}_{3}^{\dagger} = \hat{\boldsymbol{g}}^{\dagger 3} = \hat{\boldsymbol{n}}$ together with Eqs. (32) and (49) and $P_{1}(\Theta) = \Theta$, Eq. (127) becomes

$$\begin{aligned} \varepsilon \hat{\boldsymbol{H}}^{\ddagger\dagger} = & \left[ \left(\hat{\boldsymbol{x}}_{0,\alpha}^{\ddagger} - \hat{\boldsymbol{a}}_{\alpha}\right) + \left(\hat{\boldsymbol{x}}_{1,\alpha}^{\ddagger} + \frac{1}{2}\hat{\boldsymbol{a}}_{\alpha} \cdot \hat{\boldsymbol{b}}\right) P_{1}(\Theta) + \sum_{i=2}^{\infty} \hat{\boldsymbol{x}}_{i,\alpha}^{\ddagger} P_{i}(\Theta) \right] \otimes \\ & \left[ \sum_{m=0}^{\infty} \frac{1}{2^{m}} \hat{\boldsymbol{a}}^{\alpha} \cdot \hat{\boldsymbol{b}}^{m} \sum_{k=0}^{m} c_{k} \alpha_{mk} P_{k}(\Theta) \right] \\ & + \frac{2}{\delta}\left(\hat{\boldsymbol{x}}_{1}^{\ddagger} - \frac{\delta}{2}\hat{\boldsymbol{n}}\right) \otimes \boldsymbol{n} + \frac{2}{\delta}\left(\sum_{i=2}^{\infty} \hat{\boldsymbol{x}}_{i}^{\ddagger} \frac{\mathrm{d}P_{i}(\Theta)}{\mathrm{d}\Theta}\right) \otimes \boldsymbol{n} \ . \end{aligned} \tag{129}$$

Substituting Eq. (129) into the constraints in Eq. (87) yields

$$\begin{aligned} \hat{\Gamma}_{\alpha}\left(\hat{\boldsymbol{E}}^{\ddagger\dagger}\right) = & \frac{\varepsilon}{2}\left( \hat{\boldsymbol{a}}_{\alpha} \cdot \frac{2}{\delta}\left(\sum_{i=1}^{\infty} \hat{\boldsymbol{x}}_{i}^{\ddagger} \frac{\mathrm{d}P_{i}(\Theta)}{\mathrm{d}\Theta}\right) + \right. \\ & \left. \left(\hat{\boldsymbol{n}} \cdot \sum_{i=0}^{\infty} \hat{\boldsymbol{x}}_{i,\beta}^{\ddagger} P_{i}(\Theta)\right)\left(\sum_{m=0}^{\infty} \frac{1}{2^{m}} \left[\hat{b}^{m}\right]_{\alpha}^{\beta} \sum_{k=0}^{m} c_{k} \alpha_{mk} P_{k}(\Theta)\right)\right) \ , \end{aligned} \tag{130}$$

$$\hat{\Gamma}_{3}\left(\hat{\boldsymbol{E}}^{\ddagger\dagger}\right) = \varepsilon\left( \frac{2}{\delta}\left(\hat{\boldsymbol{x}}_{1}^{\ddagger} - \frac{\delta}{2}\hat{\boldsymbol{n}}\right) \cdot \hat{\boldsymbol{n}} + \frac{2}{\delta}\left(\sum_{i=2}^{\infty} \hat{\boldsymbol{x}}_{i}^{\ddagger} \frac{\mathrm{d}P_{i}(\Theta)}{\mathrm{d}\Theta}\right) \cdot \hat{\boldsymbol{n}} \right) \ . \tag{131}$$

The expressions for the constraints in Eqs. (130) and (131) can be substituted into Eq. (121) to obtain order of magnitude estimates for the reactive stresses. To this end, first note the relation between the second Piola-Kirchhoff stress $\hat{\boldsymbol{S}}_{\mathrm{r}}^{\ddagger}$ and the associated Cauchy stress $\hat{\boldsymbol{\sigma}}_{\mathrm{r}}^{\ddagger}$,

$$\hat{\boldsymbol{\sigma}}_{\mathrm{r}}^{\ddagger} = \frac{1}{\hat{J}^{\ddagger\dagger}} \hat{\boldsymbol{F}}^{\ddagger\dagger} \hat{\boldsymbol{S}}_{\mathrm{r}}^{\ddagger} \left(\hat{\boldsymbol{F}}^{\ddagger\dagger}\right)^{T} , \tag{132}$$

where $\hat{J}^{\ddagger\dagger} = \sqrt{\det \hat{\boldsymbol{C}}^{\ddagger\dagger}}$. However, from Eqs. (124), (125), (130), and (131), it follows that

$$\hat{\boldsymbol{\sigma}}_{\mathrm{r}}^{\ddagger} = \hat{\boldsymbol{S}}_{\mathrm{r}}^{\ddagger} + \mathcal{O}\left(\varepsilon^{2}\right) , \tag{133}$$

implying that the Cauchy and second Piola-Kirchhoff stresses coincide up to $\mathcal{O}\left(\varepsilon^{2}\right)$. To understand the reactive stresses in more detail, note that in the purely mechanical case the tractions $\hat{\boldsymbol{t}}^{\pm} = \hat{\boldsymbol{\sigma}}^{T}\big|_{\mathcal{S}^{\pm}} \hat{\boldsymbol{n}}$ are only affected by the reactive stresses, i.e. $\hat{\boldsymbol{t}}^{\pm} = \hat{\boldsymbol{\sigma}}_{r}^{T}\big|_{\mathcal{S}^{\pm}} \hat{\boldsymbol{n}}$ (see Sec. 4.2 of the main text). Therefore, we find

$$\hat{\boldsymbol{t}}^{\pm} = \pm \frac{1}{2} \sum_{\alpha=1}^{2} K_{\alpha} \hat{\Gamma}_{\alpha}\left(\hat{\boldsymbol{E}}^{\ddagger\dagger}\right)\bigg|_{\mathcal{S}^{\pm}} \hat{\boldsymbol{a}}_{\alpha} \pm K_{3} \hat{\Gamma}_{3}\left(\hat{\boldsymbol{E}}^{\ddagger\dagger}\right)\bigg|_{\mathcal{S}^{\pm}} \hat{\boldsymbol{n}} , \tag{134}$$

which shows that deviations from K-L kinematics must be balanced by external tractions.

Equations (130), (131), and (133) now allow making qualitative statements about the kinematics required to neglect higher-order reactive stresses in the linear momentum balance in Sec. 4.3 of the main text. From Eq. (131), we find that if

$$\left(\hat{\boldsymbol{x}}_{1}^{\ddagger} - \frac{\delta}{2} \hat{\boldsymbol{n}}\right) \cdot \hat{\boldsymbol{n}} \gg \hat{\boldsymbol{x}}_{i}^{\ddagger} \cdot \hat{\boldsymbol{n}} , \quad \forall i > 2 , \tag{135}$$

and

$$\hat{\boldsymbol{x}}_{2}^{\ddagger} \cdot \hat{\boldsymbol{n}} \gg \hat{\boldsymbol{x}}_{i}^{\ddagger} \cdot \hat{\boldsymbol{n}} , \quad \forall i > 2 , \tag{136}$$

$\hat{\boldsymbol{\sigma}}_{\mathrm{r}3}^{\ddagger} = \hat{\boldsymbol{S}}_{\mathrm{r}3}^{\ddagger}$ can be truncated at first polynomial order. In other words, we require that the reaction to the application of normal tractions is dominated by linear and quadratic deformations along the normal direction. To similarly derive the conditions for the truncation of the reactive stresses resulting from $\hat{\boldsymbol{\sigma}}_{\mathrm{r}\alpha}^{\ddagger}$, we express the position vector coefficients as

$$\hat{\boldsymbol{x}}_{i}^{\ddagger} = \hat{x}_{i}^{\ddagger\alpha} \hat{\boldsymbol{a}}_{\alpha} + \hat{x}_{i}^{\ddagger} \hat{\boldsymbol{n}} , \tag{137}$$

leading to

$$\hat{\boldsymbol{x}}_{i,\beta}^{\ddagger} \cdot \hat{\boldsymbol{n}} = \hat{x}_{i}^{\ddagger\alpha} \hat{b}_{\alpha\beta} + \hat{x}_{i,\beta}^{\ddagger} . \tag{138}$$

By assuming there exists an in-plane length scale $\ell$ characterizing the geometry, we find that if

$$\hat{\boldsymbol{x}}_{k}^{\ddagger} \cdot \hat{\boldsymbol{a}}_{\alpha} \gg \hat{\boldsymbol{x}}_{i}^{\ddagger} \cdot \hat{\boldsymbol{a}}_{\alpha} \quad k = 1, 2, \ \forall i > 2 . \tag{139}$$

$\hat{\boldsymbol{\sigma}}_{\mathrm{r}\alpha}^{\ddagger} = \hat{\boldsymbol{S}}_{\mathrm{r}\alpha}^{\ddagger}$ can be truncated at first polynomial order. Thus, similarly to Eqs. (135) and (136), we require that the reaction to in-plane tractions is dominated by linear and quadratic in-plane displacements.

Finally, recall that the penalty method converges to the method of Lagrange multipliers when the penalty parameters diverge to infinity, implying that we may consider Eq. (97) as a suitable approximation of the constrained problem in Eq. (92). Hence, if the assumptions in Eqs. (135), (136), and (139) are valid for the true body under consideration, and if the nature of the constraint stresses does not change as the penalty parameters diverge, the truncation of the stress vector $\boldsymbol{T}^3 = \boldsymbol{\sigma}_{\mathrm{r}}^T \boldsymbol{n}$ at first polynomial order in Secs. 3.3 and 4.4 of the main text is justified.

# 4 Three-Dimensional Angular Momentum Balance

In this section, we derive the general form of the angular momentum introduced in Sec. 2.3 of the main text,

$$\boldsymbol{g}_i \times \left(\boldsymbol{\sigma}^T \boldsymbol{g}^i\right) = \boldsymbol{0} \ . \tag{140}$$

Since the linear momentum balance of thin shells is commonly written in terms of stress vectors, it is convenient to express Eq. (140) as

$$\boldsymbol{g}_i \times \boldsymbol{T}^i = \boldsymbol{0} \ , \tag{141}$$

The common use of stress vectors for thin shells also provides the rationale for not starting from the usual symmetry condition of the stress tensor implied by Eq. (140).

To derive Eq. (141), consider an arbitrary subregion $\mathcal{P}$ of a body $\mathcal{B}$ with boundary $\partial\mathcal{P}$. The global form of the angular momentum balance in $\mathcal{P}$ then states [15]

$$\frac{\mathrm{d}}{\mathrm{d}t} \int_{\mathcal{P}} \boldsymbol{x} \times \rho \boldsymbol{v} \ \mathrm{d}v = \int_{\partial\mathcal{P}} \boldsymbol{x} \times \boldsymbol{t} \ \mathrm{d}a + \int_{\mathcal{P}} \boldsymbol{x} \times \boldsymbol{f} \ \mathrm{d}v \ , \tag{142}$$

where all variables have the same meaning as defined in the main text. We now rewrite the inertial term on the left-hand side of Eq. (142) as

$$\frac{\mathrm{d}}{\mathrm{d}t} \int_{\mathcal{P}} \boldsymbol{x} \times \rho \boldsymbol{v} \ \mathrm{d}v = \frac{\mathrm{d}}{\mathrm{d}t} \int_{\mathcal{P}_0} \boldsymbol{x} \times \rho_{\mathrm{r}} \boldsymbol{v} \ \mathrm{d}V \tag{143}$$

$$= \int_{\mathcal{P}_0} \boldsymbol{v} \times \rho_{\mathrm{r}} \boldsymbol{v} \ \mathrm{d}V + \int_{\mathcal{P}_0} \boldsymbol{x} \times \rho_{\mathrm{r}} \boldsymbol{a} \ \mathrm{d}V \tag{144}$$

$$= \int_{\mathcal{P}} \boldsymbol{x} \times \rho \boldsymbol{a} \ \mathrm{d}v \ , \tag{145}$$

where $\rho_{\mathrm{r}}$ denotes the density in the reference configuration $\mathcal{P}_0$.

To simplify Eq. (142) further, recall that the cross product of two arbitrary vectors $\boldsymbol{c}$ and $\boldsymbol{l}$ is a linear operation, implying that we can write it as

$$\boldsymbol{c} \times \boldsymbol{l} = \boldsymbol{W}_{\!c} \boldsymbol{l} \ , \tag{146}$$

where $\boldsymbol{W}_{\!c}$ is a skew-symmetric tensor whose components are determined by the components of $\boldsymbol{c}$ [16]. Using Cauchy's stress theorem $\boldsymbol{t} = \boldsymbol{\sigma}^T \boldsymbol{n}$, the traction term of Eq. (142) can therefore be expressed as

$$\boldsymbol{x} \times \boldsymbol{t} = \boldsymbol{W}_{\!\boldsymbol{x}} \boldsymbol{\sigma}^T \boldsymbol{n} \ . \tag{147}$$

Thus, we obtain

$$\int_{\partial\mathcal{P}} \boldsymbol{x} \times \boldsymbol{t} \,\mathrm{d}a = \int_{\mathcal{P}} \mathrm{div}\big(\boldsymbol{W}_{\boldsymbol{x}}\boldsymbol{\sigma}^T\big) \,\mathrm{d}v \tag{148}$$

$$= \int_{\mathcal{P}} \big(\boldsymbol{W}_{\boldsymbol{x}}\boldsymbol{\sigma}^T\big)_{,i}\, \boldsymbol{g}^i \,\mathrm{d}v \tag{149}$$

$$= \int_{\mathcal{P}} \boldsymbol{W}_{\boldsymbol{x},i}\boldsymbol{\sigma}^T\boldsymbol{g}^i + \boldsymbol{W}_{\boldsymbol{x}}\boldsymbol{\sigma}^T_{,i}\boldsymbol{g}^i \,\mathrm{d}v \tag{150}$$

$$= \int_{\mathcal{P}} \boldsymbol{x}_{,i} \times \big(\boldsymbol{\sigma}^T\boldsymbol{g}^i\big) + \boldsymbol{x} \times \mathrm{div}\big(\boldsymbol{\sigma}^{\boldsymbol{T}}\big) \,\mathrm{d}v \tag{151}$$

$$= \int_{\mathcal{P}} \boldsymbol{g}_i \times \big(\boldsymbol{\sigma}^T\boldsymbol{g}^i\big) + \boldsymbol{x} \times \mathrm{div}\big(\boldsymbol{\sigma}^{\boldsymbol{T}}\big) \,\mathrm{d}v \ , \tag{152}$$

where we have used the definition of the divergence of a tensor in curvilinear coordinates [16].

Substituting Eqs. (145) and (152) into Eq. (142) yields

$$\mathbf{0} = \int_{\mathcal{P}} \boldsymbol{x} \times \big(-\rho\boldsymbol{a} + \mathrm{div}\big(\boldsymbol{\sigma}^{\boldsymbol{T}}\big) + \boldsymbol{f}\big) + \boldsymbol{g}_i \times \big(\boldsymbol{\sigma}^T\boldsymbol{g}^i\big) \,\mathrm{d}v \ . \tag{153}$$

After using the linear momentum balance introduced in Sec. 2.3 of the main text and the localization theorem [7], Eq. (153) yields the general form of the angular momentum in Eq. (140).

# 5 Dimension Reduction of Balance Laws

In this section, we present a detailed derivation of the dimensionally-reduced balance laws discussed in Sec. 4 of the main text, beginning with the $(2+\delta)$-dimensional mass balance. Subsequently, we find general expressions for the stress vectors in terms of the stress tensor expansion coefficients. These expressions are then used to derive the $(2+\delta)$-dimensional linear and angular momentum balances.

## 5.1 Mass Balance

To derive the $(2+\delta)$-dimensional mass balance, we first recall the Lagrangian form of the three-dimensional mass balance introduced in Sec. 2.3 of the main text,

$$\frac{\hat{\rho}_{\mathrm{r}}}{\hat{\rho}} = \frac{\mathrm{d}\hat{v}}{\mathrm{d}\hat{V}} \ , \quad \forall \hat{\boldsymbol{x}} \in \mathcal{M} \ , \tag{154}$$

where $\mathrm{d}\hat{v}$ is an infinitesimal volume element in the current configuration with density $\hat{\rho}$, and $\mathrm{d}\hat{V}$ is the corresponding volume element in a reference configuration with density $\hat{\rho}_{\mathrm{r}}$. To introduce a suitable reference configuration for Eq. (154), we assume that if the mid-surface is flat at a point $\hat{\boldsymbol{x}}_0 \in \mathcal{S}_0$, the density is homogeneous along the thickness direction at that point. As a result, we can choose a locally flat configuration with constant density $\hat{\rho}_{\mathrm{r}}$ as reference configuration for every point $\hat{\boldsymbol{x}} \in \mathcal{M}$. In the following, we use this choice in Eq. (154) to determine the expansion of the density relative to the mid-surface density. The mid-surface density is then found using the Eulerian form of the three-dimensional mass balance,

$$\frac{\mathrm{d}\rho}{\mathrm{d}t} + \rho\,\mathrm{div}(\boldsymbol{v}) = 0 \ , \quad \forall \boldsymbol{x} \in \mathcal{M} \ , \tag{155}$$

introduced in Sec. 2.3 of the main text.

Given the K-L assumption that the membrane does not stretch along the thickness direction (see Sec. 2.1 of the main text), we can rewrite Eq. (154) as

$$\frac{\hat{\rho}_{\mathrm{r}}}{\hat{\rho}} = \frac{\mathrm{d}\hat{a}}{\mathrm{d}\hat{A}} , \quad \forall \hat{\boldsymbol{x}} \in \mathcal{M} , \tag{156}$$

with $\mathrm{d}\hat{a}$ and $\mathrm{d}\hat{A}$ being corresponding infinitesimal area elements parallel to the mid-surface in the current and reference configurations, respectively. Using standard results for K-L kinematics [2, 3, 17, 18], the relative area change can be expressed as

$$\frac{\mathrm{d}\hat{a}}{\mathrm{d}\hat{A}} = \frac{\mathrm{d}\hat{a}_0}{\mathrm{d}\hat{A}_0} \left(1 - \delta\hat{H}\Theta + \frac{\delta^2}{4}\hat{K}\Theta^2\right) , \tag{157}$$

where $\mathrm{d}\hat{a}_0$ and $\mathrm{d}\hat{A}_0$ are corresponding infinitesimal area elements on the mid-surface of the current and reference configurations, respectively. Combining Eqs. (156) and (157) yields

$$\hat{\rho} = \hat{\rho}_{\mathrm{mid}} \left(1 - \delta\hat{H}\Theta + \frac{\delta^2}{4}\hat{K}\Theta^2\right)^{-1} , \qquad \text{where} \quad \hat{\rho}_{\mathrm{mid}} = \hat{\rho}_{\mathrm{r}} \frac{\mathrm{d}\hat{A}_0}{\mathrm{d}\hat{a}_0} , \tag{158}$$

where we defined the mid-surface density $\hat{\rho}_{\mathrm{mid}}$. According to the mapping between the Lagrangian and Eulerian parametrizations in Eq. (11), all quantities in Eq. (158) can also be expressed in the Eulerian parametrization, yielding

$$\rho = \rho_{\mathrm{mid}} \left(1 - \delta H\Theta + \frac{\delta^2}{4}K\Theta^2\right)^{-1} . \tag{159}$$

Equation (159) shows that the density at every point $\boldsymbol{x} \in \mathcal{M}$ is entirely determined by the mid-surface curvatures and density. Furthermore, the right-hand side of Eq. (159) is a rational polynomial, implying that the density should be expanded as a series of the form

$$\rho = \sum_{k=0}^{\infty} \rho_k P_k(\Theta) , \tag{160}$$

to facilitate the dimension reduction procedure. Finding the coefficients $\rho_k$ requires an expression for the right-hand side of Eq. (159) in terms of Chebyshev polynomials. To that end, we introduce the non-dimensional curvatures

$$\tilde{H} = \delta H , \tag{161}$$

$$\tilde{K} = \delta^2 K , \tag{162}$$

satisfying $\tilde{H} < 1$ and $\tilde{K} < 1$ due to the assumption of small curvatures discussed in Sec. 3.3 of the main text. By recalling $\Theta \in (-1, 1)$, Taylor expanding twice yields the series expansion

$$\left(1 - \tilde{H}\Theta + \frac{1}{4}\tilde{K}\Theta^2\right)^{-1} = \sum_{k=0}^{\infty} \frac{(-1)^k}{4^k} \left(1 - \tilde{H}\Theta\right)^{-(k+1)} \tilde{K}^k \Theta^{2k} \tag{163}$$

$$= \sum_{m=0}^{\infty} \sum_{k=0}^{\infty} \frac{(-1)^k}{4^k} \binom{m+k}{m} \tilde{K}^k \tilde{H}^m \Theta^{2k+m} \ . \tag{164}$$

Equation (164) can be rewritten as

$$\left(1 - \tilde{H}\Theta + \frac{1}{4}\tilde{K}\Theta^2\right)^{-1} = \sum_{m=0}^{\infty} \sum_{k=0}^{\lfloor m/2 \rfloor} \frac{(-1)^k}{4^k} \binom{m-k}{m-2k} \tilde{K}^k \tilde{H}^{m-2k} \Theta^m \tag{165}$$

$$= \sum_{m=0}^{\infty} \sum_{k=0}^{\lfloor m/2 \rfloor} \frac{(-1)^k}{4^k} \binom{m-k}{m-2k} \tilde{K}^k \tilde{H}^{m-2k} \sum_{l=0}^{m} c_l \alpha_{ml} P_l(\Theta) \ , \tag{166}$$

where we used Eq. (46) in the last step. Taking the inner product of Eq. (158) with the $n^{\text{th}}$ Chebyshev polynomial and invoking Eqs. (160) and (166) then yields the density expansion coefficients as

$$\rho_i = \rho_{\text{mid}} \sum_{m=0}^{\infty} \sum_{k=0}^{\lfloor m/2 \rfloor} \frac{(-1)^k}{4^k} \binom{m-k}{m-2k} \tilde{K}^k \tilde{H}^{m-2k} c_i \alpha_{mi} \ . \tag{167}$$

From Eq. (167), we also obtain an order of magnitude estimate for the expansion coefficients, i.e.

$$\rho_k = \rho_{\text{mid}} \, \mathcal{O}\big(\tilde{\kappa}^k\big) \ , \qquad \text{with} \quad \tilde{\kappa} = \max_{\alpha} |\delta \kappa_\alpha| \ , \tag{168}$$

which will allow us to simplify the $(2+\delta)$-dimensional theory in subsequent derivations.

Equation (167) determines the density expansion coefficients relative to the mid-surface density $\rho_{\text{mid}}$. In the Lagrangian parametrization, the mid-surface density could be obtained from the mid-surface deformation based on its definition in Eq. (158). However, the fluid-like behavior of lipid membranes along their in-plane directions motivates the use of the Eulerian form of the mass balance in Eq. (155) to determine $\rho_{\text{mid}}$. At the same time, however, choosing $\rho_{\text{mid}}$ as the unknown in Eq. (155) proves rather inconvenient as it leads to the appearance of time derivatives of the mean and Gaussian curvatures in the $(2+\delta)$-dimensional mass balance. Instead, we choose $\rho_0$ as the unknown that is to be determined from the Eulerian mass balance. The mid-surface density $\rho_{\text{mid}}$ can then be found by setting $i = 0$ in Eq. (167).

To derive an equation determining $\rho_0$, we take the inner product of the Eulerian form of the mass balance in Eq. (155), yielding

$$\left\langle \frac{\mathrm{d}\rho}{\mathrm{d}t}, P_0(\Theta) \right\rangle + \langle \rho \operatorname{div}(\boldsymbol{v}), P_0(\Theta) \rangle = 0 \ . \tag{169}$$

The first term of Eq. (169) is found by realizing that $\mathrm{d}\theta^3/\mathrm{d}t = 0$ (see Sec. 1.1, Eq. (15)) implies that the inner product and material time derivative commute, i.e.

$$\left\langle \frac{\mathrm{d}\rho}{\mathrm{d}t}, P_0(\Theta) \right\rangle = \frac{\mathrm{d}}{\mathrm{d}t} \langle \rho, P_0(\Theta) \rangle = \frac{\mathrm{d}\rho_0}{\mathrm{d}t} \ . \tag{170}$$

To evaluate the second term of Eq. (169), we expand $\operatorname{div}(\boldsymbol{v})$ as

$$\operatorname{div}(\boldsymbol{v}) = \boldsymbol{v}_{,i} \cdot \boldsymbol{g}^i \ , \tag{171}$$

and express the velocity in Eq. (22) in terms of Chebyshev polynomials as

$$\boldsymbol{v}(\theta^i,t) = \boldsymbol{v}_0(\theta^\alpha,t)P_0(\Theta) + \frac{\delta}{2}\boldsymbol{v}_1(\theta^\alpha,t)P_1(\Theta) \tag{172}$$

$$= \left(v_0^\beta \boldsymbol{a}_\beta + v_0^3 \boldsymbol{n}\right) P_0(\Theta) + \frac{\delta}{2} v_1^\beta \boldsymbol{a}_\beta P_1(\Theta) \ . \tag{173}$$

Note that the velocity expansion in Eq. (173) implies that it is not possible to write the divergence of the velocity using the covariant derivative, i.e. $\text{div}(\boldsymbol{v}) \neq v^i\big|_i$. This is due to the choice of expressing $\boldsymbol{v}$ in the basis $\{\boldsymbol{a}_1, \boldsymbol{a}_2, \boldsymbol{n}\}$ rather than in the coordinate-induced basis $\{\boldsymbol{g}_i\}_{i=1,2,3}$. We thus begin by expanding the partial derivatives in Eq. (171) using the velocity expansion in terms of Chebyshev polynomials in Eq. (22), yielding

$$\boldsymbol{v}_{,\alpha} = \left[w^\beta_{\cdot\,\alpha}\, \boldsymbol{a}_\beta + \left(v_0^\beta b_{\beta\alpha} + v^3_{0,\alpha}\right) \boldsymbol{n}\right] P_0(\Theta) + \frac{\delta}{2}\left[v^\beta_{1:\alpha} \boldsymbol{a}_\beta + v_1^\beta b_{\beta\alpha} \boldsymbol{n}\right] P_1(\Theta) \ , \tag{174}$$

$$\boldsymbol{v}_{,3} = v_1^\alpha \boldsymbol{a}_\alpha P_0(\Theta) \ . \tag{175}$$

where we defined

$$w^\beta_{\cdot\,\alpha} = v^\beta_{0:\alpha} - v_0^3 b^\beta_\alpha \ , \tag{176}$$

with the surface covariant derivative

$$v^\beta_{0:\alpha} = v^\beta_{0,\alpha} + v_0^\gamma\, {}^0\Gamma^\beta_{\gamma\alpha} \ . \tag{177}$$

From Eqs. (174) and (175), we find that the dot products in Eq. (171) evaluate to

$$\boldsymbol{v}_{,\alpha} \cdot \boldsymbol{g}^\alpha = w^\beta_{\cdot\,\alpha} \left(\boldsymbol{a}_\beta \cdot \boldsymbol{g}^\alpha\right) + \frac{\delta}{2} v^\beta_{1:\alpha} \left(\boldsymbol{a}_\beta \cdot \boldsymbol{g}^\alpha\right) \Theta \ , \tag{178}$$

$$\boldsymbol{v}_{,3} \cdot \boldsymbol{n} = 0 \ , \tag{179}$$

and using the expansion of the contravariant basis vectors in Eq. (44) yields

$$\boldsymbol{a}_\beta \cdot \boldsymbol{g}^\alpha = \sum_{m=0}^{\infty} \frac{1}{2^m} \left[\tilde{\boldsymbol{b}}^m\right]^\alpha_\beta \Theta^m \tag{180}$$

$$= \sum_{m=0}^{\infty} \frac{1}{2^m} \left[\tilde{\boldsymbol{b}}^m\right]^\alpha_\beta \sum_{k=0}^{m} c_k \alpha_{mk} P_k(\Theta) \ , \tag{181}$$

$$\boldsymbol{a}_\beta \cdot \boldsymbol{g}^\alpha \Theta = \sum_{m=0}^{\infty} \frac{1}{2^m} \left[\tilde{\boldsymbol{b}}^m\right]^\alpha_\beta \sum_{k=0}^{m+1} c_k \alpha_{(m+1)k} P_k(\Theta) \ , \tag{182}$$

where we used Eq. (46) to express the monomials $\Theta^m$ in terms of Chebyshev polynomials. Equations (178)–(182) now show the divergence of the velocity can be written as

$$\text{div}(\boldsymbol{v}) = \sum_{m=0}^{\infty} \frac{1}{2^m} \left[\tilde{\boldsymbol{b}}^m\right]^\alpha_\beta \left( w^\beta_{\cdot\,\alpha} \sum_{k=0}^{m} c_k \alpha_{mk} P_k(\Theta) + v^\beta_{1:\alpha} \frac{\delta}{2} \sum_{k=0}^{m+1} c_k \alpha_{(m+1)k} P_k(\Theta) \right) \ . \tag{183}$$

Next, we multiply Eq. (183) by $\rho$ and use the series expansion in Eq. (160) and $P_k(\Theta)P_l(\Theta) = \frac{1}{2}\left(P_{k+l}(\Theta) + P_{|k-l|}(\Theta)\right)$ to find

$$\rho \mathrm{div}(\boldsymbol{v}) = \sum_{m=0}^{\infty} \frac{1}{2^{m+1}} \left[\tilde{\boldsymbol{b}}^m\right]^{\alpha}_{\beta} \Bigg( w^{\beta}_{.\alpha} \sum_{l=0}^{\infty}\sum_{k=0}^{m} \rho_l c_k \alpha_{mk} \left(P_{k+l}(\Theta) + P_{|k-l|}(\Theta)\right) + v^{\beta}_{1:\alpha} \frac{\delta}{2} \sum_{l=0}^{\infty}\sum_{k=0}^{m+1} \rho_l c_k \alpha_{(m+1)k} \left(P_{k+l}(\Theta) + P_{|k-l|}(\Theta)\right) \Bigg) . \tag{184}$$

This expression allows us to evaluate the inner product in Eq. (169), yielding

$$\langle \rho \mathrm{div}(\boldsymbol{v}), P_0(\Theta)\rangle = \sum_{m=0}^{\infty} \frac{1}{2^{m+1}} \left[\tilde{\boldsymbol{b}}^m\right]^{\alpha}_{\beta} \Bigg( w^{\beta}_{.\alpha} \Bigg( \rho_0 \alpha_{m0} + \sum_{k=1}^{m} \rho_k \alpha_{mk} \Bigg) + v^{\beta}_{1:\alpha} \frac{\delta}{2} \Bigg( \rho_0 \alpha_{(m+1)0} + \sum_{k=1}^{m+1} \rho_k \alpha_{(m+1)k} \Bigg) \Bigg) . \tag{185}$$

To simplify Eq. (185), we recall Eq. (168) and note that if $m-k$ is odd, $\alpha_{mk} = 0$. Thus, it is sufficient to keep the lowest order, odd terms of the summations highlighted in green in Eq. (185), reducing it to

$$\langle \rho \mathrm{div}(\boldsymbol{v}), P_0(\Theta)\rangle = \sum_{m=0}^{\infty} \frac{1}{2^{m+1}} \left[\tilde{\boldsymbol{b}}^m\right]^{\alpha}_{\beta} \Big( w^{\beta}_{.\alpha} \left(\rho_0 \alpha_{m0} + \rho_1 \alpha_{m1}\right) + v^{\beta}_{1:\alpha} \frac{\delta}{2} \left(\rho_0 \alpha_{(m+1)0} + \rho_1 \alpha_{(m+1)1}\right) \Big) + \mathcal{O}\left(\tilde{\kappa}^2\right) . \tag{186}$$

Furthermore, we can use the following relation derived in Sec. 3.3 of the main text

$$\tilde{\boldsymbol{b}}^k : \boldsymbol{A} = \mathcal{O}\left(\tilde{\kappa}^k\right)(\boldsymbol{i} : \boldsymbol{A}) = \mathcal{O}\left(\tilde{\kappa}^k\right) A^{\alpha}_{.\alpha} , \tag{187}$$

to obtain

$$\left[\tilde{\boldsymbol{b}}^{m+2}\right]^{\alpha}_{\beta} w^{\beta}_{.\alpha} \ll \left[\tilde{\boldsymbol{b}}^{m}\right]^{\alpha}_{\beta} w^{\beta}_{.\alpha} , \tag{188}$$

$$\left[\tilde{\boldsymbol{b}}^{m+2}\right]^{\alpha}_{\beta} v^{\beta}_{1:\alpha} \ll \left[\tilde{\boldsymbol{b}}^{m}\right]^{\alpha}_{\beta} v^{\beta}_{1:\alpha} . \tag{189}$$

Equations (188) and (189) permit truncating the remaining summation in Eq. (186) at $m = 1$, yielding

$$\langle \rho \mathrm{div}(\boldsymbol{v}), P_0(\Theta)\rangle = \rho_0 w^{\alpha}_{.\alpha} + \frac{\delta}{4}\rho_1 b^{\alpha}_{\beta} w^{\beta}_{.\alpha} + \frac{\delta^2}{8}\rho_0 b^{\alpha}_{\beta} v^{\beta}_{1:\alpha} + \frac{\delta}{4}\rho_1 v^{\alpha}_{1:\alpha} + \mathcal{O}\left(\tilde{\kappa}^2\right) . \tag{190}$$

As discussed in the following, all colored terms in Eq. (190) can be shown to be negligible compared to $\rho_0 w^{\alpha}_{.\alpha}$. First, the term highlighted in green is small based on Eqs. (168) and (187).

Second, we note that Eq. (168) and the assumption $\left(\delta v_1^\alpha / v_0^\beta\right)^2 \ll 1$ (see Sec. 3.3 of the main text) imply

$$\tilde{\kappa} \left| \frac{\delta v_1^\alpha}{v_0^\beta} \right| \ll 1 \ . \tag{191}$$

We may then invoke Eqs. (187) and (191) and the existence of an in-plane length scale characterizing changes of the velocity $\ell_{\mathrm{v}}$ to show that the term highlighted in orange in Eq. (190) can be disregarded. Finally, we find the term highlighted in blue in Eq. (190) to be negligible based on Eqs. (168), (187) and (191), and the characteristic length scale $\ell_{\mathrm{v}}$. This simplifies Eq. (190) to

$$\langle \rho \mathrm{div}(\boldsymbol{v}), P_0(\Theta) \rangle = \rho_0 w^\alpha_{\ .\alpha} \tag{192}$$

$$= \rho_0 \left( v^\alpha_{0:\alpha} - 2 v_0^3 H \right) \ . \tag{193}$$

By inserting Eqs. (170) and (193) into the zeroth-order mass balance in Eq. (169) and defining $\rho_{\mathrm{s}} := \delta \rho_0$, we obtain

$$\frac{\mathrm{d}\rho_{\mathrm{s}}}{\mathrm{d}t} + \rho_{\mathrm{s}} \left( v^\alpha_{0:\alpha} - 2 v H \right) = 0 \ . \tag{194}$$

From Eq. (194), we can now determine the zeroth-order density coefficient, and consequently all other density coefficients using Eq. (167). Lastly, we note that Eq. (194) is the well-known Eulerian mass balance for strictly two-dimensional surfaces [19, 20].

## 5.2 Stress Vector Expansions

The linear and angular momentum balances of thin shells are often conveniently formulated in terms of stress vectors, introduced in Sec. 4.2 of the main text. In the following, we derive the expansion coefficients of the stress vectors $\boldsymbol{T}^i$ in terms of the stress tensor expansion coefficients. To that end, we consider the series expansion

$$\boldsymbol{T}^i = \boldsymbol{\sigma}^T \boldsymbol{g}^i = \sum_{n=0}^{\infty} \boldsymbol{T}^i_n(\theta^\alpha, t) P_n(\Theta) \ . \tag{195}$$

We begin by considering the in-plane stress vectors $\boldsymbol{T}^\alpha$, and write the contravariant basis vectors $\boldsymbol{g}^\alpha$ in Eq. (49) as

$$\boldsymbol{g}^\alpha = \sum_{k=0}^{\infty} \frac{1}{\beta_k} \langle \boldsymbol{g}^\alpha, P_k(\Theta) \rangle P_k(\Theta) \ , \tag{196}$$

where

$$\beta_k = \begin{cases} 1 & \text{if } k = 0 \ , \\ \frac{1}{2} & \text{otherwise} \ , \end{cases} \tag{197}$$

as defined in Sec. 3.1 of the main text. By substituting Eq. (196) and the stress tensor expansion introduced in Sec. 3.2 of the main text,

$$\boldsymbol{\sigma}\left(\theta^i, t\right) = \sum_{k=0}^{\infty} \breve{\sigma}^{ij}_k(\theta^\alpha, t)\, \breve{\boldsymbol{g}}_i(\theta^\alpha, t) \otimes \breve{\boldsymbol{g}}_j(\theta^\alpha, t) P_k(\Theta) \ , \tag{198}$$

into Eq. (195), we obtain

$$\boldsymbol{T}^\alpha = \frac{1}{2}\sum_{n=0}^{\infty}\left(\sum_{k=0}^{n}\breve{\sigma}^{\beta j}_{n-k}\frac{1}{\beta_k}\langle \boldsymbol{g}^\alpha, P_k(\Theta)\rangle \cdot \boldsymbol{a}_\beta + \sum_{k=0}^{\infty}\breve{\sigma}^{\beta j}_{n+k}\frac{1}{\beta_k}\langle \boldsymbol{g}^\alpha, P_k(\Theta)\rangle \cdot \boldsymbol{a}_\beta + \sum_{\substack{n>0\\k=0}}^{\infty}\breve{\sigma}^{\beta j}_{k}\frac{1}{\beta_{k+n}}\langle \boldsymbol{g}^\alpha, P_{k+n}(\Theta)\rangle \cdot \boldsymbol{a}_\beta\right) P_n(\Theta)\ \breve{\boldsymbol{g}}_j \ , \tag{199}$$

where we also used $\breve{\boldsymbol{g}}_3 \cdot \boldsymbol{g}^\alpha = \boldsymbol{n}\cdot\boldsymbol{g}^\alpha = 0$. Comparison of Eqs. (195) and (199) then shows that the in-plane stress vector expansion coefficients are given by

$$\boldsymbol{T}^\alpha_n = \frac{1}{2}\left(\sum_{k=0}^{n}\breve{\sigma}^{\beta j}_{n-k}\frac{1}{\beta_k}\langle \boldsymbol{g}^\alpha, P_k(\Theta)\rangle \cdot \boldsymbol{a}_\beta + \sum_{k=0}^{\infty}\breve{\sigma}^{\beta j}_{n+k}\frac{1}{\beta_k}\langle \boldsymbol{g}^\alpha, P_k(\Theta)\rangle \cdot \boldsymbol{a}_\beta + \sum_{\substack{n>0\\k=0}}^{\infty}\breve{\sigma}^{\beta j}_{k}\frac{1}{\beta_{k+n}}\langle \boldsymbol{g}^\alpha, P_{k+n}(\Theta)\rangle \cdot \boldsymbol{a}_\beta\right) \breve{\boldsymbol{g}}_j \ . \tag{200}$$

The inner products appearing in Eq. (200) can be evaluated using Eq. (49), yielding

$$\boldsymbol{a}_\beta \cdot \frac{1}{\beta_k}\langle \boldsymbol{g}^\alpha, P_k(\Theta)\rangle = \sum_{m=0}^{\infty}\frac{1}{2^m}\left[\tilde{\boldsymbol{b}}^m\right]^\alpha_\beta c_k \alpha_{mk} \ , \tag{201}$$

which allows us to write the in-plane stress vector coefficients as

$$\boldsymbol{T}^\alpha_n = \frac{1}{2}\left(\sum_{k=0}^{n}\sigma^{\beta j}_{n-k}\sum_{m=0}^{\infty}\frac{1}{2^m}\left[\tilde{\boldsymbol{b}}^m\right]^\alpha_\beta c_k\alpha_{mk} + \sum_{k=0}^{\infty}\sigma^{\beta j}_{n+k}\sum_{m=0}^{\infty}\frac{1}{2^m}\left[\tilde{\boldsymbol{b}}^m\right]^\alpha_\beta c_k\alpha_{mk} + \sum_{\substack{n>0\\k=0}}^{\infty}\sigma^{\beta j}_{k}\sum_{m=0}^{\infty}\frac{1}{2^m}\left[\tilde{\boldsymbol{b}}^m\right]^\alpha_\beta c_{k+n}\alpha_{m(k+n)}\right) \breve{\boldsymbol{g}}_j \ , \tag{202}$$

which we introduced in Sec. 4.2 of the main text.

To evaluate the expansion coefficients of the out-of-plane stress vectors $\boldsymbol{T}^3$, we recall that $\boldsymbol{g}^3 = \boldsymbol{n}$ is independent of $\theta^3$. From Eqs. (195) and (198), we thus find

$$\boldsymbol{T}^3 = \boldsymbol{\sigma}^T\boldsymbol{n} = \sum_{n=0}^{\infty}\breve{\sigma}^{3j}_n\breve{\boldsymbol{g}}_j P_n(\Theta) \ . \tag{203}$$

implying that the expansion coefficients of $\boldsymbol{T}^3$ are given by

$$\boldsymbol{T}^3_n = \breve{\sigma}^{3j}_n\breve{\boldsymbol{g}}_j \ , \tag{204}$$

as discussed in Sec. 4.2 of the main text.

From the form of the stress vector coefficients in Eq. (204) and the order of magnitude assumptions for the reactive stresses discussed in Sec. 3.3 of the main text, we find that the zeroth- and first-order expansion coefficients of $\boldsymbol{T}^3$ dominate all others, i.e.

$$\boldsymbol{T}^3_k \gg \boldsymbol{T}^3_l \ , \quad k = 0, 1 \ , \ \forall l \geq 2 \ . \tag{205}$$

To obtain a similar result for the in-plane stress vector coefficients $\boldsymbol{T}^\alpha_n$, we recall the following order of magnitude estimate derived in Sec. 3.3 of the main text,

$$\boldsymbol{c} \cdot (\delta \boldsymbol{b})^m \, \boldsymbol{a}^\alpha = \boldsymbol{c} \cdot \boldsymbol{i} \boldsymbol{a}^\alpha \, \mathcal{O}((\delta\kappa)^m) \ , \tag{206}$$

where $\boldsymbol{c} = c^\gamma \boldsymbol{l}_\gamma$ is an arbitrary vector written in terms of the orthonormal eigenvectors of the curvature tensor $\boldsymbol{l}_\gamma$. By invoking Eq. (206) and the stress assumptions discussed in Sec. 3.3 of the main text, we find that the order of magnitude of $\boldsymbol{T}^\alpha_n$, $n \geq 2$, is not larger than the order of magnitude of $\boldsymbol{T}^\alpha_0$ and $\boldsymbol{T}^\alpha_1$.

## 5.3 Linear Momentum Balance

In this section, we apply the dimension reduction method to the three-dimensional linear momentum balance introduced in Sec. 2.3 of the main text,

$$\rho \dot{\boldsymbol{v}} = \operatorname{div}\big(\boldsymbol{\sigma}^T\big) + \boldsymbol{f} \ , \quad \forall \boldsymbol{x} \in \mathcal{M} \ . \tag{207}$$

To simplify the following derivations, we consider each term of Eq. (207) individually.

**Inertia** To obtain the inertial contribution on the left-hand side of Eq. (207) in terms of Chebyshev polynomials, we first derive an expression for the acceleration $\boldsymbol{a} = \dot{\boldsymbol{v}}$. To this end, recall the definition of the material time derivative as

$$\dot{\boldsymbol{v}}\big(\theta^i, t\big) = \frac{\mathrm{d}}{\mathrm{d}t} \boldsymbol{v}\big(\theta^i, t\big) = \frac{\partial}{\partial t} \boldsymbol{v}\big(\theta^i, t\big)\bigg|_{\xi^k} \ . \tag{208}$$

When applying the material time derivative to the velocity expansion in Eq. (172) to find the acceleration $\boldsymbol{a}$, i.e.

$$\boldsymbol{a} = \dot{\boldsymbol{v}} = \big(\dot{v}^\alpha_0 \boldsymbol{a}_\alpha + v^\alpha_0 \dot{\boldsymbol{a}}_\alpha + \dot{v}^3_0 \boldsymbol{n} + v^3_0 \dot{\boldsymbol{n}}\big) \, P_0(\Theta) + \frac{\delta}{2} \left(\dot{v}^\alpha_1 \boldsymbol{a}_\alpha + v^\alpha_1 \dot{\boldsymbol{a}}_\alpha\right) P_1(\Theta) \ , \tag{209}$$

we require expressions for the material time derivatives of the velocity components and basis vectors. However, the material time derivative of quantities transforming co- or contravariantly does not coincide with their total time derivative [21]. Using Eq. (28) along with results derived in Refs. [21] and [22, Ch. 5.1 (c)], we instead find

$$\dot{v}^\alpha_0 = v^\alpha_{0,t} \tag{210}$$

$$\dot{v}^\alpha_1 = v^\alpha_{1,t} + v^\beta_0 v^\alpha_{1:\beta} - v^\beta_1 v^\alpha_{0,\beta} \ , \tag{211}$$

$$\dot{v}^3_0 = v^3_{0,t} + v^3_{0,\alpha} v^\alpha_0 \ , \tag{212}$$

$$\dot{\boldsymbol{a}}_\alpha = \boldsymbol{v}_{0,\alpha} \ , \tag{213}$$

with

$$\boldsymbol{v}_{0,\alpha} = \left( v^\beta_{0:\alpha} - v^3_0 b^\beta_\alpha \right) \boldsymbol{a}_\beta + \left( v^3_{0,\alpha} + v^\beta_0 b_{\beta\alpha} \right) \boldsymbol{n} \ . \tag{214}$$

By combining Eqs. (24) and (209)–(214), we obtain an expression for the acceleration under the assumption of K-L kinematics,

$$\begin{aligned} \boldsymbol{a} = \ & \left\{ \left( v^\alpha_{0,t} + v^\beta_0 v^\alpha_{0:\beta} - 2 v^3_0 v^\beta_0 b^\alpha_\beta - v^3_0 v^3_{0,\beta}\, a^{\alpha\beta} \right) \boldsymbol{a}_\alpha + \left( v^3_{0,t} + 2 v^\alpha_0 v^3_{0,\alpha} + v^\alpha_0 v^\beta_0 b_{\beta\alpha} \right) \boldsymbol{n} \right\} P_0(\Theta) \, + \\ & \frac{\delta}{2} \left\{ \left( v^\alpha_{1,t} + v^\beta_0 v^\alpha_{1,\beta} + v^\beta_1 v^\alpha_{0:\beta} - v^\beta_1 v^3_0 b^\alpha_\beta - v^\beta_1 v^\alpha_{0,\beta} \right) \boldsymbol{a}_\alpha + \left( v^\alpha_1 v^3_{0,\alpha} + v^\alpha_1 v^\beta_0 b_{\beta\alpha} \right) \boldsymbol{n} \right\} P_1(\Theta) \ . \end{aligned} \tag{215}$$

The complexity of this expression motivates the introduction of a short-hand notation. To that end, we take the material time derivative of the velocity expansion in Eq. (172) to find

$$\begin{aligned} \boldsymbol{a} = \dot{\boldsymbol{v}} &= \dot{\boldsymbol{v}}_0 P_0(\Theta) + \frac{\delta}{2} \dot{\boldsymbol{v}}_1 P_1(\Theta) && (216) \\ &= \dot{\boldsymbol{v}}_0 P_0(\Theta) + \frac{\delta}{2} \ddot{\boldsymbol{n}} P_1(\Theta) \ , && (217) \end{aligned}$$

with the second equality following from Eq. (8). By comparing Eq. (217) to Eq. (215), we identify $\dot{\boldsymbol{v}}_0$ and $\ddot{\boldsymbol{n}}$ as

$$\begin{aligned} \dot{\boldsymbol{v}}_0 &= \left( v^\alpha_{0,t} + v^\beta_0 v^\alpha_{0:\beta} - 2 v^3_0 v^\beta_0 b^\alpha_\beta - v^3_0 v^3_{0,\beta}\, a^{\alpha\beta} \right) \boldsymbol{a}_\alpha + \left( v^3_{0,t} + 2 v^\alpha_0 v^3_{0,\alpha} + v^\alpha_0 v^\beta_0 b_{\beta\alpha} \right) \boldsymbol{n} \ , && (218) \\ \ddot{\boldsymbol{n}} &= \left( v^\alpha_{1,t} + v^\beta_0 v^\alpha_{1,\beta} + v^\beta_1 v^\alpha_{0:\beta} - v^\beta_1 v^3_0 b^\alpha_\beta - v^\beta_1 v^\alpha_{0,\beta} \right) \boldsymbol{a}_\alpha + \left( v^\alpha_1 v^3_{0,\alpha} + v^\alpha_1 v^\beta_0 b_{\beta\alpha} \right) \boldsymbol{n} \ . && (219) \end{aligned}$$

Finally, multiplying Eq. (217) by the density expansion in Eq. (160) yields the series expansion of the inertial term of the linear momentum balance,

$$\begin{aligned} \rho \boldsymbol{a} &= \left( \sum_{k=0}^{\infty} \rho_k P_k(\Theta) \right) \left( \dot{\boldsymbol{v}}_0 P_0(\Theta) + \frac{\delta}{2} \ddot{\boldsymbol{n}} P_1(\Theta) \right) && (220) \\ &= \dot{\boldsymbol{v}}_0 \sum_{k=0}^{\infty} \rho_k P_k(\Theta) + \frac{\delta}{4} \ddot{\boldsymbol{n}} \sum_{k=0}^{\infty} \rho_k \left( P_{k+1}(\Theta) + P_{|k-1|}(\Theta) \right) \ . && (221) \end{aligned}$$

where we used $P_k(\Theta) P_l(\Theta) = \frac{1}{2} \left( P_{k+l}(\Theta) + P_{|k-l|}(\Theta) \right)$. Taking the inner product of Eq. (221) with the zeroth- and first-order Chebyshev polynomials results in[3]

$$\begin{aligned} \langle \delta \rho \boldsymbol{a}, P_0(\Theta) \rangle &= \dot{\boldsymbol{v}}_0 \rho_{\mathrm{s}} + \frac{\delta^2}{4} \ddot{\boldsymbol{n}} \rho_1 && (222) \\ &\approx \dot{\boldsymbol{v}}_0 \rho_{\mathrm{s}} \ , && (223) \\ 2 \langle \delta \rho \boldsymbol{a}, P_1(\Theta) \rangle &= \dot{\boldsymbol{v}}_0 \delta \rho_1 + \frac{\delta}{4} \ddot{\boldsymbol{n}} \left( 2 \rho_{\mathrm{s}} + \delta \rho_2 \right) && (224) \\ &\approx \dot{\boldsymbol{v}}_0 \delta \rho_1 + \frac{\rho_{\mathrm{s}} \delta}{2} \ddot{\boldsymbol{n}} \ , && (225) \end{aligned}$$

[3] To derive the $(2+\delta)$-dimensional equations of motion, it is sufficient to consider only the zeroth- and first-order terms of the linear momentum balance. This motivates taking the inner products with $P_0(\Theta)$ and $P_1(\Theta)$ specifically.

where the term highlighted in green in Eqs. (223) is small compared to $\dot{\boldsymbol{v}}_0\rho_\mathrm{s}$ based on Eqs. (168), (191), (218), and (219), and the existence of a characteristic in-plane velocity length scale $\ell_\mathrm{v}$. Furthermore, the pre-factor of 2 in Eq. (225) originates from $\langle P_1(\Theta), P_1(\Theta)\rangle = 1/2$, and the term highlighted in blue is negligible since Eq. (167) implies $\delta\rho_2 \ll \rho_\mathrm{s}$. Equation (225) can be simplified further by noting that according to Eq. (167),

$$\rho_0 = \rho_\mathrm{mid}\left(1 + \mathcal{O}\big(\tilde{\kappa}^2\big)\right) \ , \tag{226}$$

$$\rho_1 = \rho_\mathrm{mid}\left(\delta H + \mathcal{O}\big(\tilde{\kappa}^3\big)\right) \ , \tag{227}$$

thus implying

$$\rho_1 \approx \rho_0 \delta H \ . \tag{228}$$

Hence, by combining Eqs. (223), (225), and (228), we finally obtain

$$\delta\rho\boldsymbol{a} \overset{1}{\approx} \rho_\mathrm{s}\dot{\boldsymbol{v}}_0 P_0(\Theta) + \left(\rho_\mathrm{s}\delta H\dot{\boldsymbol{v}}_0 + \frac{\delta\rho_\mathrm{s}}{2}\,\ddot{\boldsymbol{n}}\right) P_1(\Theta) \ , \tag{229}$$

where $\overset{1}{\approx}$ indicates truncation at first polynomial order.

**Stress divergence** To derive the $(2+\delta)$-dimensional form of the stress term in Eq. (207), we first write the stress divergence in terms of the stress vectors $\boldsymbol{T}^i$,

$$\operatorname{div}\big(\boldsymbol{\sigma}^T\big) = \big(\boldsymbol{\sigma}^T\big)_{,i}\,\boldsymbol{g}^i = \big(\boldsymbol{\sigma}^T\boldsymbol{g}^i\big)_{,i} - \boldsymbol{\sigma}^T\boldsymbol{g}^i_{,i} = \boldsymbol{T}^i_{,i} + \boldsymbol{T}^j\Gamma^i_{ji} = \boldsymbol{T}^i\big|_i \ , \tag{230}$$

where $\boldsymbol{T}^i\big|_i$ is the covariant derivative of $\boldsymbol{T}^i$. Given the expressions for the Christoffel symbols in Eqs. (50)–(53), we can now rewrite the stress vector divergence $\boldsymbol{T}^i\big|_i$ as

$$\boldsymbol{T}^i\big|_i = \boldsymbol{T}^\alpha_{,\alpha} + \boldsymbol{T}^3_{,3} + \boldsymbol{T}^\alpha\Gamma^\beta_{\alpha\beta} + \boldsymbol{T}^3\Gamma^\beta_{3\beta} \ . \tag{231}$$

By using the stress vector expansion in Eq. (195), the partial derivatives in Eq. (231) evaluate to

$$\boldsymbol{T}^\alpha_{,\alpha} = \sum_{k=0}^{\infty}\boldsymbol{T}^\alpha_{k,\alpha}P_k(\Theta) \ , \tag{232}$$

$$\boldsymbol{T}^3_{,3} = \frac{2}{\delta}\sum_{k=1}^{\infty}k\boldsymbol{T}^3_k U_{k-1}(\Theta) \ , \tag{233}$$

where $U_k(\Theta)$ indicates the $k^\mathrm{th}$ Chebyshev polynomial of the second kind. These can be expressed in terms of the Chebyshev polynomials of the first kind [23] as

$$\boldsymbol{T}^3_{,3} = \frac{2}{\delta}\sum_{k=1}^{\infty}k\boldsymbol{T}^3_k\begin{cases}2\sum_{j=0}^{(k-2)/2}P_{2j+1}(\Theta) \ , & \text{even } k \ ,\\ 2\sum_{j=0}^{(k-1)/2}P_{2j}(\Theta) - 1 \ , & \text{odd } k \ .\end{cases} \tag{234}$$

Taking the inner product of Eqs. (232) and (234) with the zeroth- and first-order Chebyshev polynomial yields

$$\langle\boldsymbol{T}^\alpha_{,\alpha}, P_0(\Theta)\rangle = \boldsymbol{T}^\alpha_{0,\alpha} \ , \tag{235}$$

$$2\,\langle \boldsymbol{T}^{\alpha}_{,\alpha}, P_1(\Theta)\rangle = \boldsymbol{T}^{\alpha}_{1,\alpha} \ , \tag{236}$$

$$\langle \boldsymbol{T}^{3}_{,3}, P_0(\Theta)\rangle = \frac{2}{\delta}\sum_{k=1}^{\infty}(2k-1)\boldsymbol{T}^{3}_{2k-1} \ , \tag{237}$$

$$2\,\langle \boldsymbol{T}^{3}_{,3}, P_1(\Theta)\rangle = \frac{4}{\delta}\sum_{k=1}^{\infty} 2k\boldsymbol{T}^{3}_{2k} \ . \tag{238}$$

Next, we expand the first of the terms involving the Christoffel symbols in Eq. (231). Using the generic series expansion of the stress vector in Eq. (195) and the expression for the Christoffel symbol in Eq. (61), we find

$$\boldsymbol{T}^{\alpha}\,\Gamma^{\beta}_{\alpha\beta} = \left(\sum_{l=0}^{\infty}\boldsymbol{T}^{\alpha}_{l}P_l(\Theta)\right)\left({}^{0}\Gamma^{\beta}_{\alpha\beta} - \frac{1}{2}\sum_{m=0}^{\infty}\frac{1}{2^m}\boldsymbol{a}^{\beta}\cdot\tilde{\boldsymbol{b}}^{m}\boldsymbol{a}_{\gamma}\,\tilde{b}^{\gamma}_{\alpha;\beta}\sum_{k=0}^{m+1}c_k\alpha_{(m+1)k}P_k(\Theta)\right) \tag{239}$$

$$= \sum_{l=0}^{\infty}\boldsymbol{T}^{\alpha}_{l}\,{}^{0}\Gamma^{\beta}_{\alpha\beta}P_l(\Theta)$$

$$- \frac{1}{4}\sum_{m=0}^{\infty}\frac{1}{2^m}\boldsymbol{a}^{\beta}\cdot\tilde{\boldsymbol{b}}^{m}\boldsymbol{a}_{\gamma}\,\tilde{b}^{\gamma}_{\alpha;\beta}\sum_{l=0}^{\infty}\sum_{k=0}^{m+1}\boldsymbol{T}^{\alpha}_{l}c_k\alpha_{(m+1)k}\left(P_{k+l}(\Theta) + P_{|k-l|}(\Theta)\right) \ , \tag{240}$$

and taking the same inner products as before yields

$$\langle \boldsymbol{T}^{\alpha}\,\Gamma^{\beta}_{\alpha\beta}, P_0(\Theta)\rangle = \boldsymbol{T}^{\alpha}_{0}\,{}^{0}\Gamma^{\beta}_{\alpha\beta} - \frac{1}{4}\sum_{m=0}^{\infty}\frac{1}{2^m}\boldsymbol{a}^{\beta}\cdot\tilde{\boldsymbol{b}}^{m}\boldsymbol{a}_{\gamma}\,\tilde{b}^{\gamma}_{\alpha;\beta}\sum_{k=0}^{m+1}\boldsymbol{T}^{\alpha}_{k}\alpha_{(m+1)k} \ , \tag{241}$$

$$2\,\langle \boldsymbol{T}^{\alpha}\,\Gamma^{\beta}_{\alpha\beta}, P_1(\Theta)\rangle = \boldsymbol{T}^{\alpha}_{1}\,{}^{0}\Gamma^{\beta}_{\alpha\beta} -$$

$$\frac{1}{4}\sum_{m=0}^{\infty}\frac{1}{2^m}\boldsymbol{a}^{\beta}\cdot\tilde{\boldsymbol{b}}^{m}\boldsymbol{a}_{\gamma}\,\tilde{b}^{\gamma}_{\alpha;\beta}\sum_{k=0}^{m+1}c_k\alpha_{(m+1)k}\left(\boldsymbol{T}^{\alpha}_{k+1} + \frac{1}{c_{|k-1|}}\boldsymbol{T}^{\alpha}_{|k-1|}\right) \ . \tag{242}$$

Similarly, using the expression for the Christoffel symbol $\Gamma^{\alpha}_{3\alpha}$ in Eq. (65), we can express the second Christoffel symbol term in Eq. (231) as

$$\boldsymbol{T}^{3}\Gamma^{\beta}_{3\beta} = \left(\sum_{k=0}^{\infty}\boldsymbol{T}^{3}_{k}P_k(\Theta)\right)\left(-\frac{2}{\delta}\sum_{m=1}^{\infty}\frac{1}{2^m}\operatorname{tr}\left(\tilde{\boldsymbol{b}}^{m}\right)\sum_{l=0}^{m-1}c_l\alpha_{(m-1)l}P_l(\Theta)\right) \tag{243}$$

$$= -\frac{1}{\delta}\sum_{m=1}^{\infty}\frac{1}{2^m}\operatorname{tr}\left(\tilde{\boldsymbol{b}}^{m}\right)\sum_{k=0}^{\infty}\sum_{l=0}^{m-1}\boldsymbol{T}^{3}_{k}c_l\alpha_{(m-1)l}\left(P_{l+k}(\Theta) + P_{|l-k|}(\Theta)\right) \ , \tag{244}$$

and taking the usual inner products leads to

$$\langle \boldsymbol{T}^{3}\Gamma^{\beta}_{3\beta}, P_0(\Theta)\rangle = -\frac{1}{\delta}\sum_{m=1}^{\infty}\frac{1}{2^m}\operatorname{tr}\left(\tilde{\boldsymbol{b}}^{m}\right)\sum_{k=0}^{m-1}\boldsymbol{T}^{3}_{k}\alpha_{(m-1)k} \ , \tag{245}$$

$$2\,\langle \boldsymbol{T}^{3}\Gamma^{\beta}_{3\beta}, P_1(\Theta)\rangle = -\frac{1}{\delta}\sum_{m=1}^{\infty}\frac{1}{2^m}\operatorname{tr}\left(\tilde{\boldsymbol{b}}^{m}\right)\sum_{k=0}^{m-1}c_k\alpha_{(m-1)k}\left(\boldsymbol{T}^{3}_{k+1} + \frac{1}{c_{|k-1|}}\boldsymbol{T}^{3}_{|k-1|}\right) \ . \tag{246}$$

Combining the results in Eqs. (235)–(238), (241), (242), (245), and (246) yields the stress divergence contribution to the linear momentum balance,

$$\boldsymbol{T}^i\big|_i \stackrel{1}{=} P_0(\Theta)\left\{\boldsymbol{T}^\alpha_{0:\alpha} - \frac{1}{4}\sum_{m=0}^{\infty}\frac{1}{2^m}\boldsymbol{a}^\beta\cdot\tilde{\boldsymbol{b}}^m\boldsymbol{a}_\gamma\,\tilde{b}^\gamma_{\alpha;\beta}\sum_{k=0}^{m+1}\boldsymbol{T}^\alpha_k\alpha_{(m+1)k} + \frac{2}{\delta}\sum_{k=1}^{\infty}(2k-1)\boldsymbol{T}^3_{2k-1} - \frac{1}{\delta}\sum_{m=1}^{\infty}\frac{1}{2^m}\operatorname{tr}\left(\tilde{\boldsymbol{b}}^m\right)\sum_{k=0}^{m-1}\boldsymbol{T}^3_k\alpha_{(m-1)k}\right\} + P_1(\Theta)\left\{\boldsymbol{T}^\alpha_{1:\alpha} - \frac{1}{4}\sum_{m=0}^{\infty}\frac{1}{2^m}\boldsymbol{a}^\beta\cdot\tilde{\boldsymbol{b}}^m\boldsymbol{a}_\gamma\,\tilde{b}^\gamma_{\alpha;\beta}\sum_{k=0}^{m+1}c_k\alpha_{(m+1)k}\left(\boldsymbol{T}^\alpha_{k+1} + \frac{1}{c_{|k-1|}}\boldsymbol{T}^\alpha_{|k-1|}\right) + \frac{4}{\delta}\sum_{k=1}^{\infty}2k\boldsymbol{T}^3_{2k} - \frac{1}{\delta}\sum_{m=1}^{\infty}\frac{1}{2^m}\operatorname{tr}\left(\tilde{\boldsymbol{b}}^m\right)\sum_{k=0}^{m-1}c_k\alpha_{(m-1)k}\left(\boldsymbol{T}^3_{k+1} + \frac{1}{c_{|k-1|}}\boldsymbol{T}^3_{|k-1|}\right)\right\}\ , \tag{247}$$

where $\stackrel{1}{=}$ again indicates truncation at first polynomial order. To simplify Eq. (247), we note that the terms highlighted in blue are of the form of the contraction in Eq. (187). Furthermore, we recall the assumption that the order of magnitude of the stress vectors does not increase with increasing order (see Sec. 3.3 of the main text). Therefore, it is sufficient to retain the terms highlighted in blue only up to $m = 1$, yielding

$$\sum_{m=0}^{\infty}\frac{1}{2^m}\boldsymbol{a}^\beta\cdot\tilde{\boldsymbol{b}}^m\boldsymbol{a}_\gamma\,\tilde{b}^\gamma_{\alpha;\beta}\sum_{k=0}^{m+1}\boldsymbol{T}^\alpha_k\alpha_{(m+1)k} \approx 2\tilde{H}_{,\alpha}\boldsymbol{T}^\alpha_1 + \frac{1}{2}\tilde{b}^\beta_\gamma\tilde{b}^\gamma_{\alpha;\beta}\left(\boldsymbol{T}^\alpha_0 + \frac{1}{2}\boldsymbol{T}^\alpha_2\right)\ , \tag{248}$$

and

$$\sum_{m=0}^{\infty}\frac{1}{2^m}\boldsymbol{a}^\beta\cdot\tilde{\boldsymbol{b}}^m\boldsymbol{a}_\gamma\,\tilde{b}^\gamma_{\alpha;\beta}\sum_{k=0}^{m+1}c_k\alpha_{(m+1)k}\left(\boldsymbol{T}^\alpha_{k+1} + \frac{1}{c_{|k-1|}}\boldsymbol{T}^\alpha_{|k-1|}\right) \approx 2\tilde{H}_{,\alpha}\left(2\boldsymbol{T}^\alpha_0 + \boldsymbol{T}^\alpha_2\right) + \frac{1}{4}\tilde{b}^\beta_\gamma\tilde{b}^\gamma_{\alpha;\beta}\left(3\boldsymbol{T}^\alpha_1 + \boldsymbol{T}^\alpha_3\right)\ , \tag{249}$$

where we used the Mainardi-Codazzi relation $\tilde{b}^\beta_{\alpha;\beta} = 2\tilde{H}_{,\alpha}$. Similarly, we may use the result (see Eq. (187))

$$\operatorname{tr}\left(\tilde{\boldsymbol{b}}^m\right) = \mathcal{O}(\tilde{\kappa}^m)\ , \tag{250}$$

and the assumption that the reactive stresses are dominated by their zeroth- and first-order contributions to truncate the terms highlighted in green in Eq. (247), simplifying them to

$$\sum_{m=1}^{\infty}\frac{1}{2^m}\operatorname{tr}\left(\tilde{\boldsymbol{b}}^m\right)\sum_{k=0}^{m-1}\boldsymbol{T}^3_k\alpha_{(m-1)k} = \sum_{m=1}^{\infty}\frac{1}{2^m}\operatorname{tr}\left(\tilde{\boldsymbol{b}}^m\right)\left(\boldsymbol{T}^3_0\alpha_{(m-1)0} + \boldsymbol{T}^3_1\alpha_{(m-1)1}\right) \tag{251}$$

$$\approx 2\tilde{H}\boldsymbol{T}^3_0 + \frac{1}{4}\operatorname{tr}\left(\tilde{\boldsymbol{b}}^2\right)\boldsymbol{T}^3_1\ , \tag{252}$$

and

$$\sum_{m=1}^{\infty} \frac{1}{2^m} \operatorname{tr}\left(\tilde{\boldsymbol{b}}^m\right) \sum_{k=0}^{m-1} c_k \alpha_{(m-1)k} \left(\boldsymbol{T}^3_{k+1} + \frac{1}{c_{|k-1|}} \boldsymbol{T}^3_{|k-1|}\right)$$
$$\approx \sum_{m=1}^{\infty} \frac{1}{2^m} \operatorname{tr}\left(\tilde{\boldsymbol{b}}^m\right) \left(\alpha_{(m-1)0} \boldsymbol{T}^3_1 + 2\alpha_{(m-1)1} \boldsymbol{T}^3_0\right) \tag{253}$$
$$\approx 2\tilde{H}\boldsymbol{T}^3_1 + \frac{1}{2} \operatorname{tr}\left(\tilde{\boldsymbol{b}}^2\right) \boldsymbol{T}^3_0 \; , \tag{254}$$

where we also used $\operatorname{tr} \tilde{\boldsymbol{b}} = 2\tilde{H}$.

Substituting Eqs. (248), (249), (252) and (254) reduces Eq. (247) to

$$\boldsymbol{T}^i\big|_i \overset{1}{\approx} P_0(\Theta) \Bigg\{ \boldsymbol{T}^\alpha_{0:\alpha} - \frac{1}{2}\tilde{H}_{,\alpha}\boldsymbol{T}^\alpha_1 - \frac{1}{8}\tilde{b}^\beta_\gamma \tilde{b}^\gamma_{\alpha;\beta}\left(\boldsymbol{T}^\alpha_0 + \frac{1}{2}\boldsymbol{T}^\alpha_2\right) + \frac{2}{\delta}\sum_{k=1}^{\infty}(2k-1)\boldsymbol{T}^3_{2k-1}$$
$$- \frac{2}{\delta}\tilde{H}\boldsymbol{T}^3_0 - \frac{1}{4\delta}\operatorname{tr}\left(\tilde{\boldsymbol{b}}^2\right)\boldsymbol{T}^3_1 \Bigg\} +$$
$$P_1(\Theta) \Bigg\{ \boldsymbol{T}^\alpha_{1:\alpha} - \frac{1}{2}\tilde{H}_{,\alpha}\left(2\boldsymbol{T}^\alpha_0 + \boldsymbol{T}^\alpha_2\right) - \frac{1}{16}\tilde{b}^\beta_\gamma \tilde{b}^\gamma_{\alpha;\beta}\left(3\boldsymbol{T}^\alpha_1 + \boldsymbol{T}^\alpha_3\right) +$$
$$\frac{4}{\delta}\sum_{k=1}^{\infty} 2k\boldsymbol{T}^3_{2k} - \frac{2}{\delta}\tilde{H}\boldsymbol{T}^3_1 - \frac{1}{2\delta}\operatorname{tr}\left(\tilde{\boldsymbol{b}}^2\right)\boldsymbol{T}^3_0 \Bigg\} \; . \tag{255}$$

The terms highlighted in green in Eq. (255) can be neglected based on Eq. (187), the condition (see Sec. 3.3 of the main text)

$$\frac{\ell_c}{\ell_s} \lll 1 \; , \tag{256}$$

and the assumption that the order of magnitude of the stresses does not increase with polynomial order. Furthermore, the term highlighted in orange is negligible based on the assumption that the reactive stresses are dominated by their zeroth- and first-order coefficients. The latter assumption also suggests that we may truncate the term highlighted in blue at first order such that we obtain

$$\boldsymbol{T}^i\big|_i \overset{1}{\approx} P_0(\Theta) \left\{ \boldsymbol{T}^\alpha_{0:\alpha} - \frac{1}{2}\tilde{H}_{,\alpha}\boldsymbol{T}^\alpha_1 + \frac{2}{\delta}\boldsymbol{T}^3_1 - \frac{2}{\delta}\tilde{H}\boldsymbol{T}^3_0 - \frac{1}{4\delta}\operatorname{tr}\left(\tilde{\boldsymbol{b}}^2\right)\boldsymbol{T}^3_1 \right\} +$$
$$P_1(\Theta) \left\{ \boldsymbol{T}^\alpha_{1:\alpha} - \frac{1}{2}\tilde{H}_{,\alpha}\left(2\boldsymbol{T}^\alpha_0 + \boldsymbol{T}^\alpha_2\right) - \frac{2}{\delta}\tilde{H}\boldsymbol{T}^3_1 - \frac{1}{2\delta}\operatorname{tr}\left(\tilde{\boldsymbol{b}}^2\right)\boldsymbol{T}^3_0 \right\} \; . \tag{257}$$

Finally, based on Eq. (250), we find that the term highlighted in green is small. By additionally using the result

$$\operatorname{tr}\left(\tilde{\boldsymbol{b}}^2\right) = 2\left(2\tilde{H}^2 - \tilde{K}\right) \; , \tag{258}$$

Eq. (257) simplifies to

$$\boldsymbol{T}^i\big|_i \overset{1}{\approx} P_0(\Theta)\left\{\boldsymbol{T}^\alpha_{0:\alpha} - \frac{1}{2}\tilde{H}_{,\alpha}\boldsymbol{T}^\alpha_1 + \frac{2}{\delta}\boldsymbol{T}^3_1 - \frac{2}{\delta}\tilde{H}\boldsymbol{T}^3_0\right\} + P_1(\Theta)\left\{\boldsymbol{T}^\alpha_{1:\alpha} - \tilde{H}_{,\alpha}\left(\boldsymbol{T}^\alpha_0 + \frac{1}{2}\boldsymbol{T}^\alpha_2\right) - \frac{2}{\delta}\tilde{H}\boldsymbol{T}^3_1 - \frac{1}{\delta}\left(2\tilde{H}^2 - \tilde{K}\right)\boldsymbol{T}^3_0\right\} \tag{259}$$

$$= P_0(\Theta)\left\{\boldsymbol{T}^\alpha_{0:\alpha} - \frac{\delta}{2}H_{,\alpha}\boldsymbol{T}^\alpha_1 + \frac{2}{\delta}\boldsymbol{T}^3_1 - 2H\boldsymbol{T}^3_0\right\} + P_1(\Theta)\left\{\boldsymbol{T}^\alpha_{1:\alpha} - \delta H_{,\alpha}\left(\boldsymbol{T}^\alpha_0 + \frac{1}{2}\boldsymbol{T}^\alpha_2\right) - 2H\boldsymbol{T}^3_1 - \delta\left(2H^2 - K\right)\boldsymbol{T}^3_0\right\} , \tag{260}$$

which is the expression for the stress divergence term used in Sec. 4.3 of the main text.

**Body force term** For simplicity, we assume in the main text that the body force $\boldsymbol{f}$ is defined per unit volume rather than per unit mass. This makes the body force independent of other quantities and motivates the use of the generic series

$$\boldsymbol{f} = \sum_{k=0}^{\infty} \boldsymbol{f}_k P_k(\Theta) , \tag{261}$$

implying

$$\langle \boldsymbol{f}, P_0(\Theta)\rangle = \boldsymbol{f}_0 , \tag{262}$$

$$2\langle \boldsymbol{f}, P_1(\Theta)\rangle = \boldsymbol{f}_1 , \tag{263}$$

and

$$\boldsymbol{f} \overset{1}{=} \boldsymbol{f}_0 P_0(\Theta) + \boldsymbol{f}_1 P_1(\Theta) . \tag{264}$$

## 5.4 Angular Momentum Balance

To derive the $(2+\delta)$-dimensional angular momentum balance, we start from the three-dimensional angular momentum balance in Eq. (141). Upon substituting Eq. (49), $\boldsymbol{g}_3 = \boldsymbol{n}$, and the stress vector expansion in Eq. (195) into Eq. (141), we find

$$\boldsymbol{0} = \boldsymbol{g}_i \times \boldsymbol{T}^i = \left(\boldsymbol{a}_\alpha P_0(\Theta) - \frac{1}{2}\tilde{b}^\beta_\alpha \boldsymbol{a}_\beta P_1(\Theta)\right) \times \left(\sum_{i=0}^{\infty} \boldsymbol{T}^\alpha P_k(\Theta)\right) + \boldsymbol{n} \times \left(\sum_{i=0}^{\infty} \boldsymbol{T}^3 P_k(\Theta)\right) \tag{265}$$

$$= \sum_{k=0}^{\infty} \boldsymbol{a}_\alpha \times \boldsymbol{T}^\alpha_k P_k(\Theta) + \sum_{k=0}^{\infty} \boldsymbol{n} \times \boldsymbol{T}^3_k P_k(\Theta) - \sum_{k=0}^{\infty} \boldsymbol{a}_\beta \times \frac{1}{4}\tilde{b}^\beta_\alpha \boldsymbol{T}^\alpha \left(P_{k+1}(\Theta) + P_{|k-1|}(\Theta)\right) . \tag{266}$$

Taking the dot product of Eq. (266) with the normal vector leads to the condition,

$$\sum_{k=0}^{\infty} \boldsymbol{T}^\alpha_k \cdot \boldsymbol{a}^\beta P_k(\Theta) - \frac{1}{4}\tilde{b}^\alpha_\gamma \sum_{k=0}^{\infty} \boldsymbol{T}^\gamma_k \cdot \boldsymbol{a}^\beta \left(P_{k+1}(\Theta) + P_{|k-1|}(\Theta)\right) \quad \text{is symmetric} , \tag{267}$$

and taking the inner product with the $n^{\text{th}}$ Chebsyhev polynomial reduces Eq. (267) to

$$\boldsymbol{T}_n^\alpha \cdot \boldsymbol{a}^\beta - \frac{1}{4}\tilde{b}_\gamma^\alpha \left(\boldsymbol{T}_{n+1}^\gamma + \boldsymbol{T}_{|n-1|}^\gamma\right) \cdot \boldsymbol{a}^\beta \quad \text{is symmetric,} \quad \forall n \in \mathbb{N}_0 \ . \tag{268}$$

By taking the dot product of Eq. (266) with the covariant tangent vector $\boldsymbol{a}_\beta$, we can write the in-plane components of Eq. (266) as

$$\sum_{k=0}^{\infty} \boldsymbol{T}_k^\alpha \cdot \boldsymbol{n}\, P_k(\Theta) - \frac{1}{4}\tilde{b}_\gamma^\alpha \sum_{k=0}^{\infty} \boldsymbol{T}_k^\gamma \cdot \boldsymbol{n} \left(P_{k+1}(\Theta) + P_{|k-1|}(\Theta)\right) - \sum_{k=0}^{\infty} \boldsymbol{T}_k^3 \cdot \boldsymbol{a}^\alpha\, P_k(\Theta) = 0 \ . \tag{269}$$

Taking the inner product of Eq. (269) with the $n^{\text{th}}$ Chebyshev polynomial then yields the condition

$$\boldsymbol{T}_n^\alpha \cdot \boldsymbol{n} - \frac{1}{4}\tilde{b}_\gamma^\alpha \left(\boldsymbol{T}_{n+1}^\gamma + \boldsymbol{T}_{|n-1|}^\gamma\right) \cdot \boldsymbol{n} - \boldsymbol{T}_n^3 \cdot \boldsymbol{a}^\alpha = 0 \ , \quad \forall n \in \mathbb{N}_0 \ . \tag{270}$$

We can now relate Eqs. (268) and (270) to the usual symmetry condition of the Cauchy stress tensor,

$$\boldsymbol{\sigma}^T = \boldsymbol{\sigma} \ , \tag{271}$$

which, according to Sec. 4, is equivalent to Eq. (141). Direct comparison shows that Eq. (271) can be expressed in component form as

$$\varepsilon_{ijk} \breve{\sigma}^{ij} \breve{\boldsymbol{g}}^k = 0 \ . \tag{272}$$

Furthermore, by using $\boldsymbol{g}_i = \left(\boldsymbol{g}_i \cdot \breve{\boldsymbol{g}}^j\right) \breve{\boldsymbol{g}}_j$ and $\boldsymbol{g}^i = \left(\boldsymbol{g}^i \cdot \breve{\boldsymbol{g}}_j\right) \breve{\boldsymbol{g}}^j$, it is found that the stress vector form of the angular momentum balance in Eq. (141) is equal to Eq. (272) as well. Therefore, taking the dot products of Eq. (272) with the normal vector $\boldsymbol{n}$ and in-plane basis vectors $\boldsymbol{a}_\alpha$ shows that Eqs. (267) and (269) are respectively identical to

$$\breve{\sigma}^{\alpha\beta} = \breve{\sigma}^{\beta\alpha} \ , \tag{273}$$

$$\breve{\sigma}^{\alpha 3} = \breve{\sigma}^{3\alpha} \ . \tag{274}$$

After taking the inner product with the $n^{\text{th}}$ Chebyshev polynomial, we further find that Eqs. (268) and (270) are respectively identical to

$$\breve{\sigma}_n^{\alpha\beta} = \breve{\sigma}_n^{\beta\alpha} \ , \quad \forall n \in \mathbb{N}_0 \ , \tag{275}$$

$$\breve{\sigma}_n^{\alpha 3} = \breve{\sigma}_n^{3\alpha} \ , \quad \forall n \in \mathbb{N}_0 \ . \tag{276}$$

Equation (275) implies that the normal component of the dimensionally-reduced angular momentum balance is satisfied to arbitrary order if the three-dimensional, in-plane components of the stress tensor satisfy the usual symmetry condition in Eq. (271). Similarly, the symmetry of the reactive stresses discussed in Sec. 2.3 of the main text implies that Eq. (276) is satisfied a-priori. Finally, we note that Eqs. (275) and (276) also follow from algebraically tedious manipulations of Eqs. (268) and (270).

## References


[1] Omar, Y. A. D., Lipel, Z. G. & Mandadapu, K. K. The $(2 + \delta)$-dimensional theory of the electromechanics of lipid membranes: I. Electrostatics (2023). arXiv:2301.09610.

[2] Naghdi, P. M. Foundations of elastic shell theory. Tech. Rep., Institute of Engineering Research, University of California (1962).

[3] Song, Z. & Dai, H.-H. On a consistent finite-strain shell theory based on 3-D nonlinear elasticity. *International Journal of Solids and Structures* **97**, 137–149 (2016).

[4] Cody, W. A survey of practical rational and polynomial approximation of functions. *SIAM Review* **12**, 400–423 (1970).

[5] Nocedal, J. & Wright, S. J. *Numerical optimization* (Springer, 1999).

[6] Ciarlet, P. G. *Mathematical elasticity: Three-dimensional elasticity* (SIAM, 2021).

[7] Gurtin, M. E., Fried, E. & Anand, L. *The mechanics and thermodynamics of continua* (Cambridge university press, 2010).

[8] Ugural, A. C. *Stresses in beams, plates, and shells* (CRC press, 2009).

[9] Ciarlet, P. G. & Destuynder, P. Justification of the two-dimensional linear plate model. *Journal de Mécanique* **18**, 315–344 (1979).

[10] Ciarlet, P. G. A justification of the von Kármán equations. *Archive for Rational Mechanics and Analysis* **73**, 349–389 (1980).

[11] Podio-Guidugli, P. An exact derivation of the thin plate equation. *Journal of Elasticity* **22**, 121–133 (1989).

[12] Podio-Guidugli, P. Constraint and scaling methods to derive shell theory from three-dimensional elasticity. *Rivista di Matematica della Universita di Parma* **16**, 73–83 (1990).

[13] Miara, B. Justification of the asymptotic analysis of elastic plates, I. The linear case. *Asymptotic Analysis* **9**, 47–60 (1994).

[14] Miara, B. Justification of the asymptotic analysis of elastic plates, II. The non-linear case. *Asymptotic Analysis* **9**, 119–134 (1994).

[15] Chadwick, P. *Continuum mechanics: concise theory and problems* (Courier Corporation, 1999).

[16] Itskov, M. *Tensor algebra and tensor analysis for engineers* (Springer, 2019).

[17] Chien, W.-Z. The intrinsic theory of thin shells and plates. I. General theory. *Quarterly of Applied Mathematics* **1**, 297–327 (1944).

[18] Green, A. & Zerna, W. The equilibrium of thin elastic shells. *The Quarterly Journal of Mechanics and Applied Mathematics* **3**, 9–22 (1950).

[19] Scriven, L. E. Dynamics of a fluid interface equation of motion for Newtonian surface fluids. *Chemical Engineering Science* **12**, 98–108 (1960).

[20] Sahu, A., Sauer, R. A. & Mandadapu, K. K. Irreversible thermodynamics of curved lipid membranes. *Physical Review E* **96**, 042409 (2017).

[21] Oldroyd, J. G. On the formulation of rheological equations of state. *Proceedings of the Royal Society of London. Series A. Mathematical and Physical Sciences* **200**, 523–541 (1950).

[22] Sahu, A. *Irreversible Thermodynamics and Hydrodynamics of Biological Membranes*. Ph.D. thesis, University of California, Berkeley (2022).

[23] Boyd, J. P. *Chebyshev and Fourier spectral methods* (Courier Corporation, 2001).
